# Supplementary material for: Impact of Noisy Supervision in Foundation Model Learning
Source: arXiv:2403.06869 source file (2025-05-05)
Supplement: Supplementary file 1 [file sec-appendix.tex]

\section{Understanding the Noisy Labels in Pre-training Data}
\label{sec:append-understand}

We provide additional experiment details for the motivating example of ResNet-50 in this section.  
We also present the detailed results on each downstream dataset for noisy pre-trained models on both ImageNet-1K and YFCC15M. 
The SVD plots on each dataset are also shown here.

\subsection{Pre-training Datasets and Hyper-parameters}
\label{sec:append-understand-setup}

For analysis in \cref{sec:understand}, we conduct pre-training of ResNet-50 on ImageNet-1K and YFCC15M. 

For ImageNet-1K pre-training, we follow the training recipe in \cite{wightman2021resnet}. 
To introduce noise in ImageNet-1K, we use function cleanlab \citep{northcutt2021confidentlearning} to introduce symmetric noise in each class. 
For YFCC15M CLIP pre-training, we follow the training recipe in \cite{cherti2023reproducible}. 
To introduce noise in YFCC15M, we swap the text description between two randomly sampled image-text pairs until the noise ratio is achieved. 
We show the validation accuracy on ImageNet-1K of the noisy ResNet-50 models pre-trained on ImageNet-1K and zero-shot accuracy on ImageNet-1K of the noisy ResNet-50 models pre-trained on YFCC15M  in \cref{tab:r50-imagenet-acc}.
The results show that our pre-training achieves the state-of-the-art results \citep{wightman2021resnet,cherti2023reproducible}, as a basis for our further analysis.

\begin{table}[h]
\centering
\caption{ImageNet-1K validation and zero-shot accuracy of ImageNet-1K pre-trained and YFCC15M CLIP pre-trained noisy ResNet-50 models.}
\label{tab:r50-imagenet-acc}
\resizebox{0.6\textwidth}{!}{%
\begin{tabular}{@{}c|c|c@{}}
\toprule
\multirow{2}{*}{Noise Ratio} & ImageNet-1K Pre-train & YFCC15M CLIP Pre-train \\
                             & Validation Accuracy   & Zero-shot Accuracy     \\ \midrule
0\%                          &    79.96                   &     32.64                   \\
5\%                          &    79.18                   &      30.86                 \\
10\%                         &    78.61                   &      29.54                  \\
20\%                         &    76.27                   &       27.72                 \\
30\%                         &    73.11                   &         26.53               \\ \bottomrule
\end{tabular}%
}
\end{table}

\subsection{Downstream Vision Datasets and Hyper-parameters}
\label{sec:append-understand-down-setup}

We present the details of the in-domain (ID) vision datasets in \cref{tab:append-exp-vision-id} and out-of-domain vision datasets \cref{tab:append-exp-vision-odd}.
For ID, we conduct training on the training set and test on the validation set of the downstream dataset.
For OOD on DomainNet \citep{peng2019moment}, we conduct training on the training set of DomainNet Real or DomainNet Sketch, and test on all the other three DomainNet datasets not used in training. 
For OOD on ImageNet \citep{ILSVRC15}, we conduct training on ImageNet training split and test on its variants.

To transfer a pre-trained model, we use linear probing (LP) for analysis as shown in \cref{sec:understand}. 
We train the linear classifier for 30 epochs on each downstream dataset, using AdamW \citep{kingma2014adam} optimizer with a cosine scheduler. We do not use weight decay for linear probing and set the learning rate to $0.1$ for all tasks. 

\begin{table}[h]
\centering
\caption{Details of the 14 in-domain (ID) vision datasets used to evaluate ID transfer performance of vision models.}
\label{tab:append-exp-vision-id}
\resizebox{0.9\textwidth}{!}{%
\begin{tabular}{l|cccc}
\toprule
\multicolumn{1}{c|}{Dataset} &  Classes & Train Size & Test Size & Evaluation Metric \\ \hline
CIFAR-10 \citep{krizhevsky2009learning}                    &            10 & 50,000 & 10,000   & accuracy           \\ 
CIFAR-100  \citep{krizhevsky2009learning}                   &          100 & 50,000 & 10,000    & accuracy                     \\
Flowers102 \citep{nilsback2008automated}               &       102 & 2,040 & 6,149            & mean per class       \\ 
Food101 \citep{FeiFei2004LearningGV}                    &    101 & 75,750 & 25,250       & accuracy               \\ 
OxfordPet \citep{parkhi12a}                    &           37 & 3,680 & 3,669          & mean per class            \\
StanfordCars  \citep{jonathan2013cars}              &       196 & 8,144 & 8,041         & accuracy              \\ 
FGVCAircraft  \citep{maji2013finegrained}              &    102 & 6,667 & 3,333         & mean per class               \\ 
SVHN  \citep{2011svhn}              &           10 & 73,257 & 26,032   & accuracy     \\ 
DTD  \citep{cimpoi14describing}              &          47 & 1,880 & 1,880           & accuracy        \\ 
Caltech101  \citep{FeiFei2004LearningGV}              &     102 & 3,060 & 6,084       & mean per class               \\ 
EuroSAT  \citep{helber2019eurosat}              &     10 & 21,600 & 5,400       & accuracy            \\ 
PatchCamelyon  \citep{Veeling2018qh}              &      10 & 73,257 & 26,032     & accuracy     \\ 
RESISC45  \citep{Cheng2017resic}              &          45 & 25,200 & 6,300       & accuracy                \\ 
Rendered SST2  \citep{socher2013recursive}              &     2 & 6,920 & 1,821         & accuracy                 \\ 
\bottomrule
\end{tabular}%
}
\end{table}

\begin{table}[h]
\centering
\caption{Details of the 4 out-of-domain (OOD) DomainNet datasets and 6 out-of-domain (OOD) ImageNet variants used to evaluate OOD transfer performance of vision models.}
\label{tab:append-exp-vision-odd}
\resizebox{0.9\textwidth}{!}{%
\begin{tabular}{l|cccc}
\toprule
\multicolumn{1}{c|}{Dataset} & Classes & Train Size & Test Size & Evaluation Metric \\ \hline
DomainNet Sketch \citep{peng2019moment}                            &          345 & 48,212 & 20,916                   & accuracy              \\ 
DomainNet Real \citep{peng2019moment}                              &      345 & 120,906 & 52,041                   &       accuracy          \\
DomainNet Painting \citep{peng2019moment}                         &           345 & - & 21,850                 &        accuracy        \\ 
DomainNet Clipart \citep{peng2019moment}                         &         345 & - & 14,604                  &            accuracy     \\ \hline
ImageNet-V2 \citep{recht2019imagenet}                         &        1,000             &     -     &     10,000                &        accuracy          \\ 
ImageNet-R \citep{dan2021ood}                  &              200       &               -  &            30,000        &           accuracy \\ 
ImageNet-Sketch \citep{wang2019learning}                         &   1,000                  &      -   &      50,889               &             accuracy      \\ 
ImageNet-A \citep{dan2021ood}                           &     200                &           -   &       7,500              &          accuracy    \\ 
ImageNet-ViD \citep{vaishaal2021time}                           &    1,000                 &     -    &                     &            accuracy       \\ 
ObjectNet \citep{objectnet2019}                               &      112               &        -    &       18,574              &         accuracy       \\ 
\bottomrule
\end{tabular}%
}
\end{table}

\subsection{Detailed ID and OOD Linear Probing Results}
\label{sec:append-id-ood-eval}

We present the detailed ID and OOD linear probing results we analyzed in \cref{sec:understand} here. 

The ImageNet-1K and YFCC15M pre-trained ID results are in \cref{fig:append-in1k-r50-id-eval} and \cref{fig:append-yfcc15m-r50-id-eval} respectively. 
On all the datasets, we can observe that the $5\%$ or $10\%$ noise pre-trained models outperform the clean pre-trained models, no matter which pre-training dataset and method is used. 

The OOD results are in \cref{fig:append-in1k-r50-ood-eval} and \cref{fig:append-yfcc15m-r50-odd-eval} respectively. On the validation split of the training dataset (ID), the trend follows the ID observations, where $5\%$ noisy pre-trained model is better. 
However, on the OOD datasets, the model performance deteriorates as noise increases. 

\begin{figure}[h]
    \centering
    \includegraphics[width=0.97\textwidth]{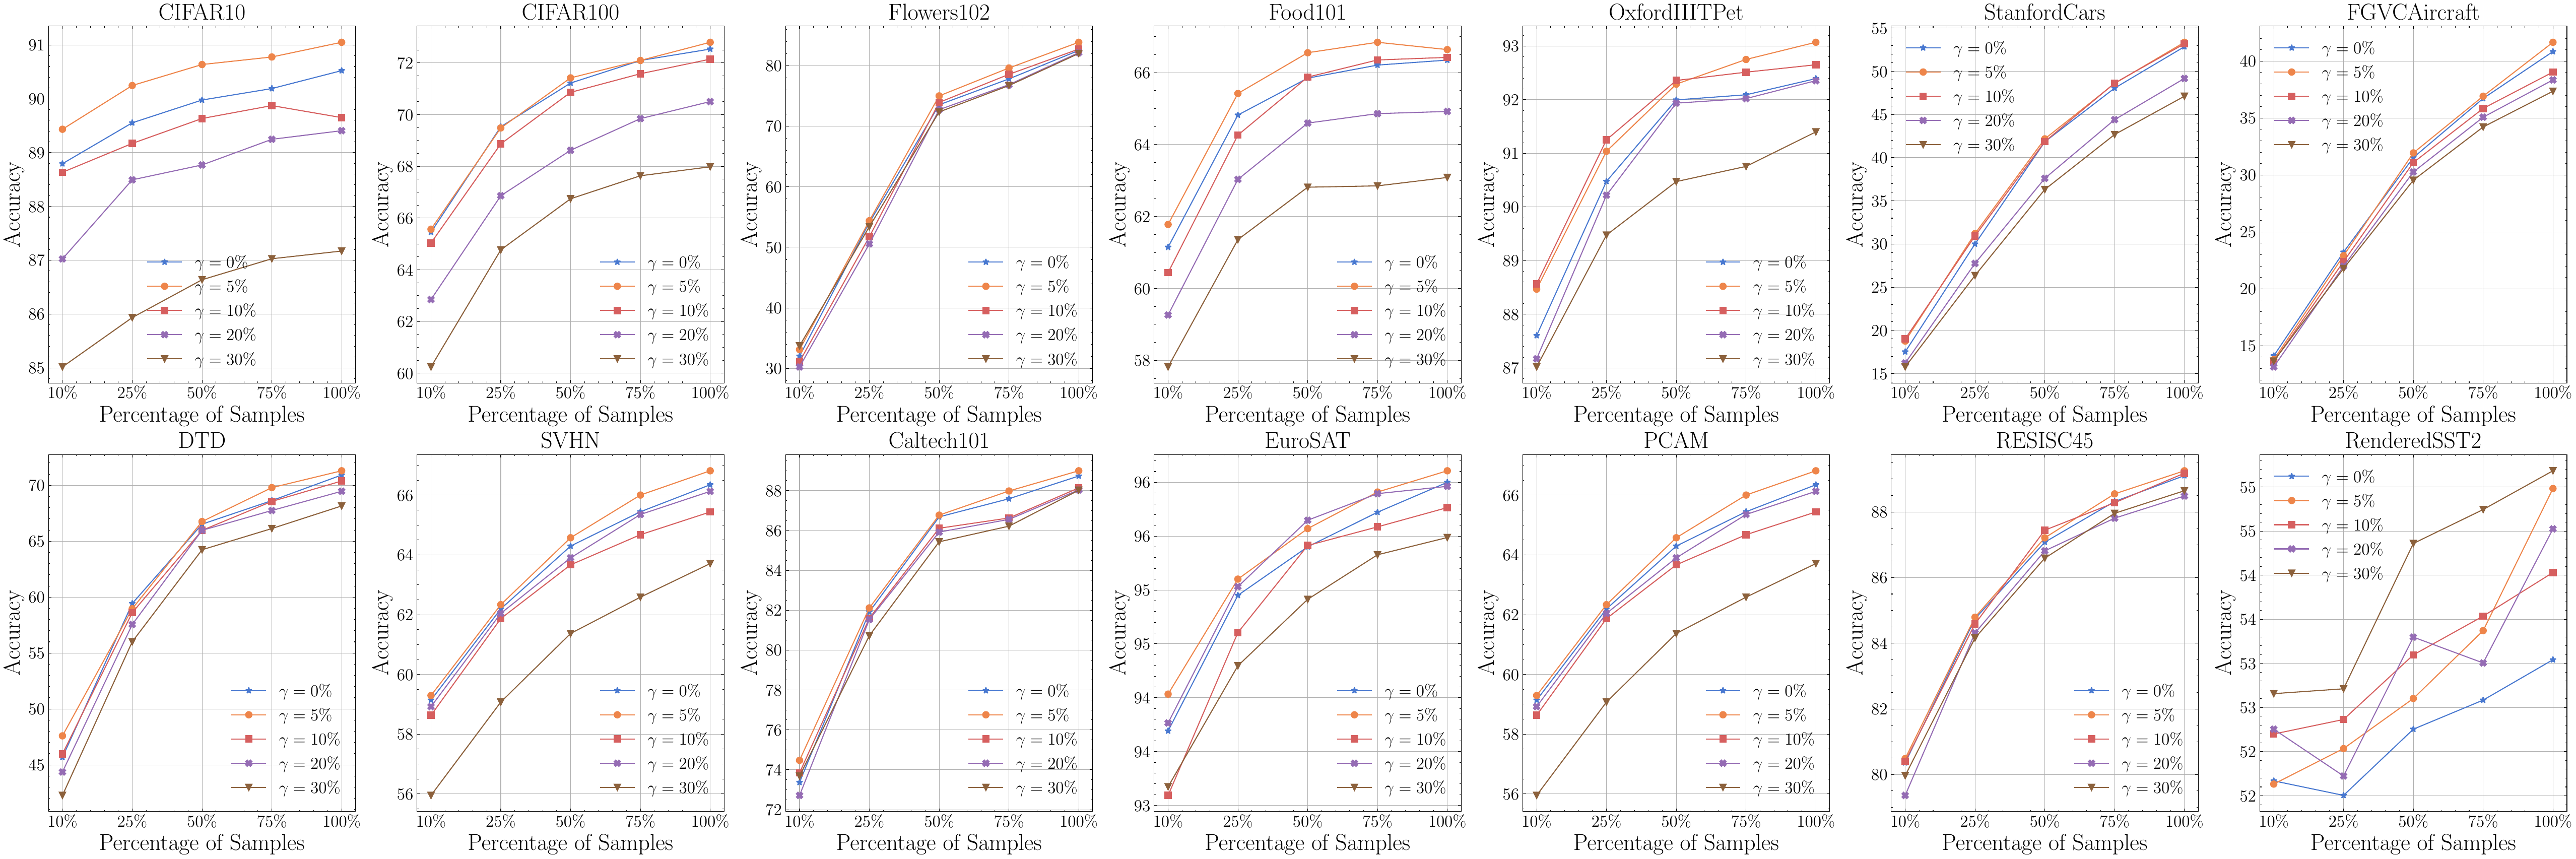}
    \caption{ImageNet-1K pre-trained ResNet-50 in-domain (ID) evaluation results}
    \label{fig:append-in1k-r50-id-eval}
\end{figure}

\begin{figure}[h]
    \centering
    \includegraphics[width=0.6\textwidth]{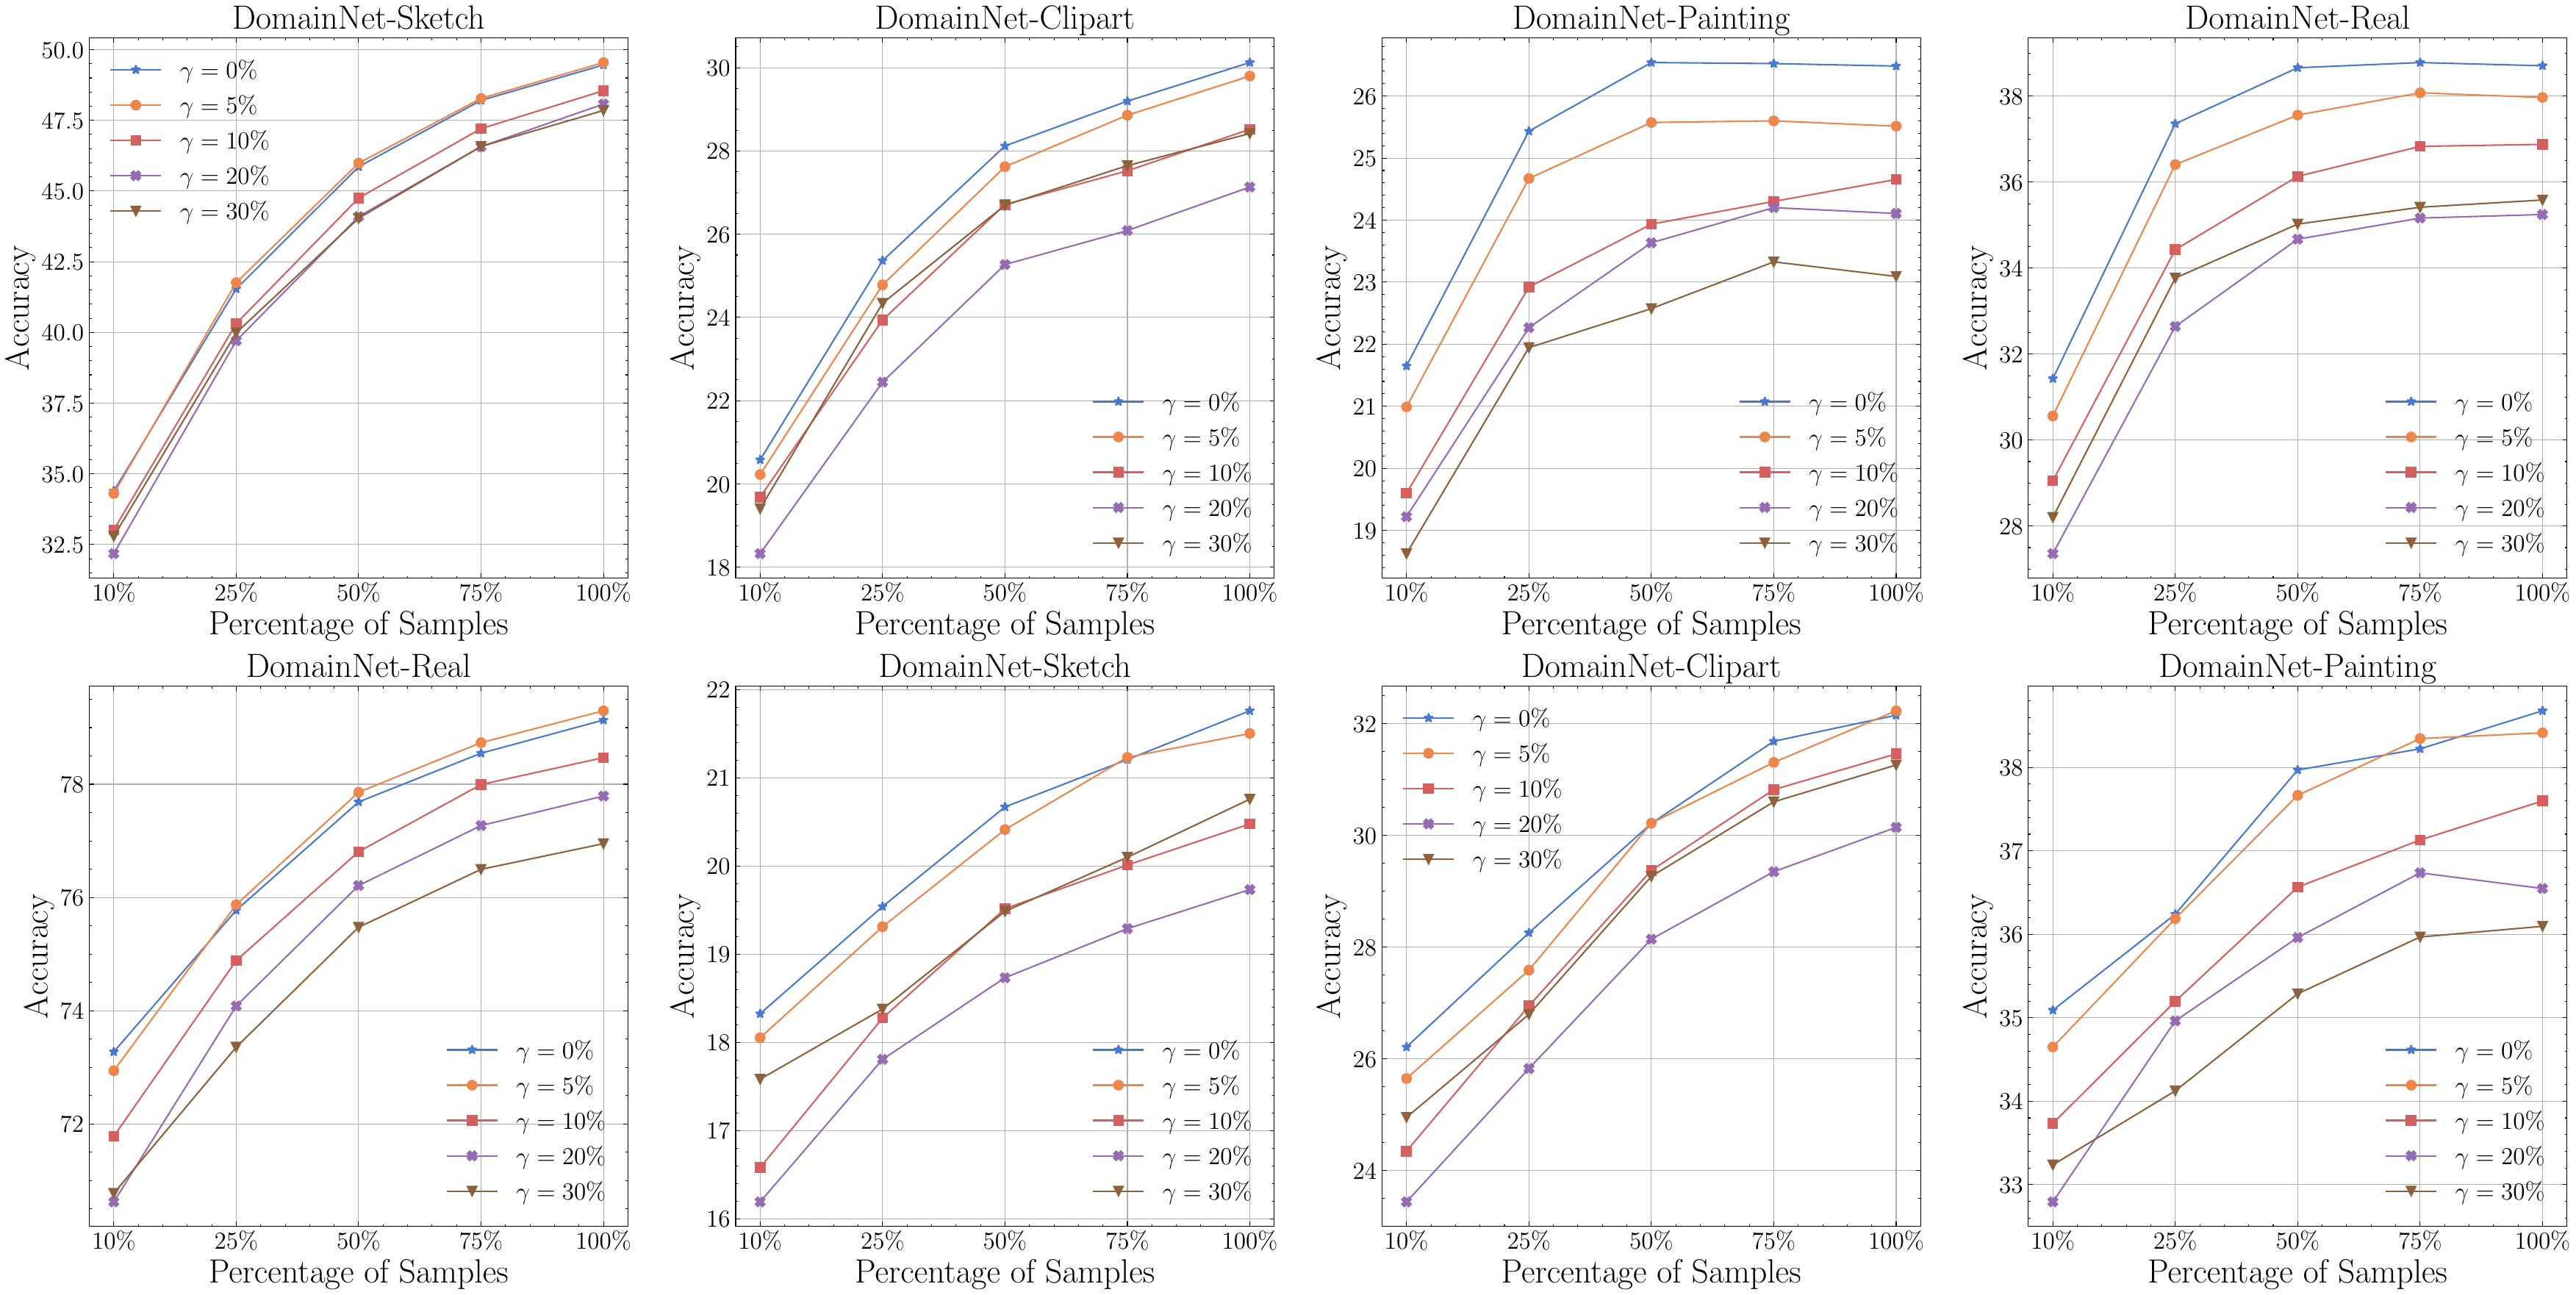}
    \caption{ImageNet-1K pre-trained ResNet-50 out-of-domain (OOD) evaluation results}
    \label{fig:append-in1k-r50-ood-eval}
\end{figure}

\begin{figure}[h]
    \centering
    \includegraphics[width=0.97\textwidth]{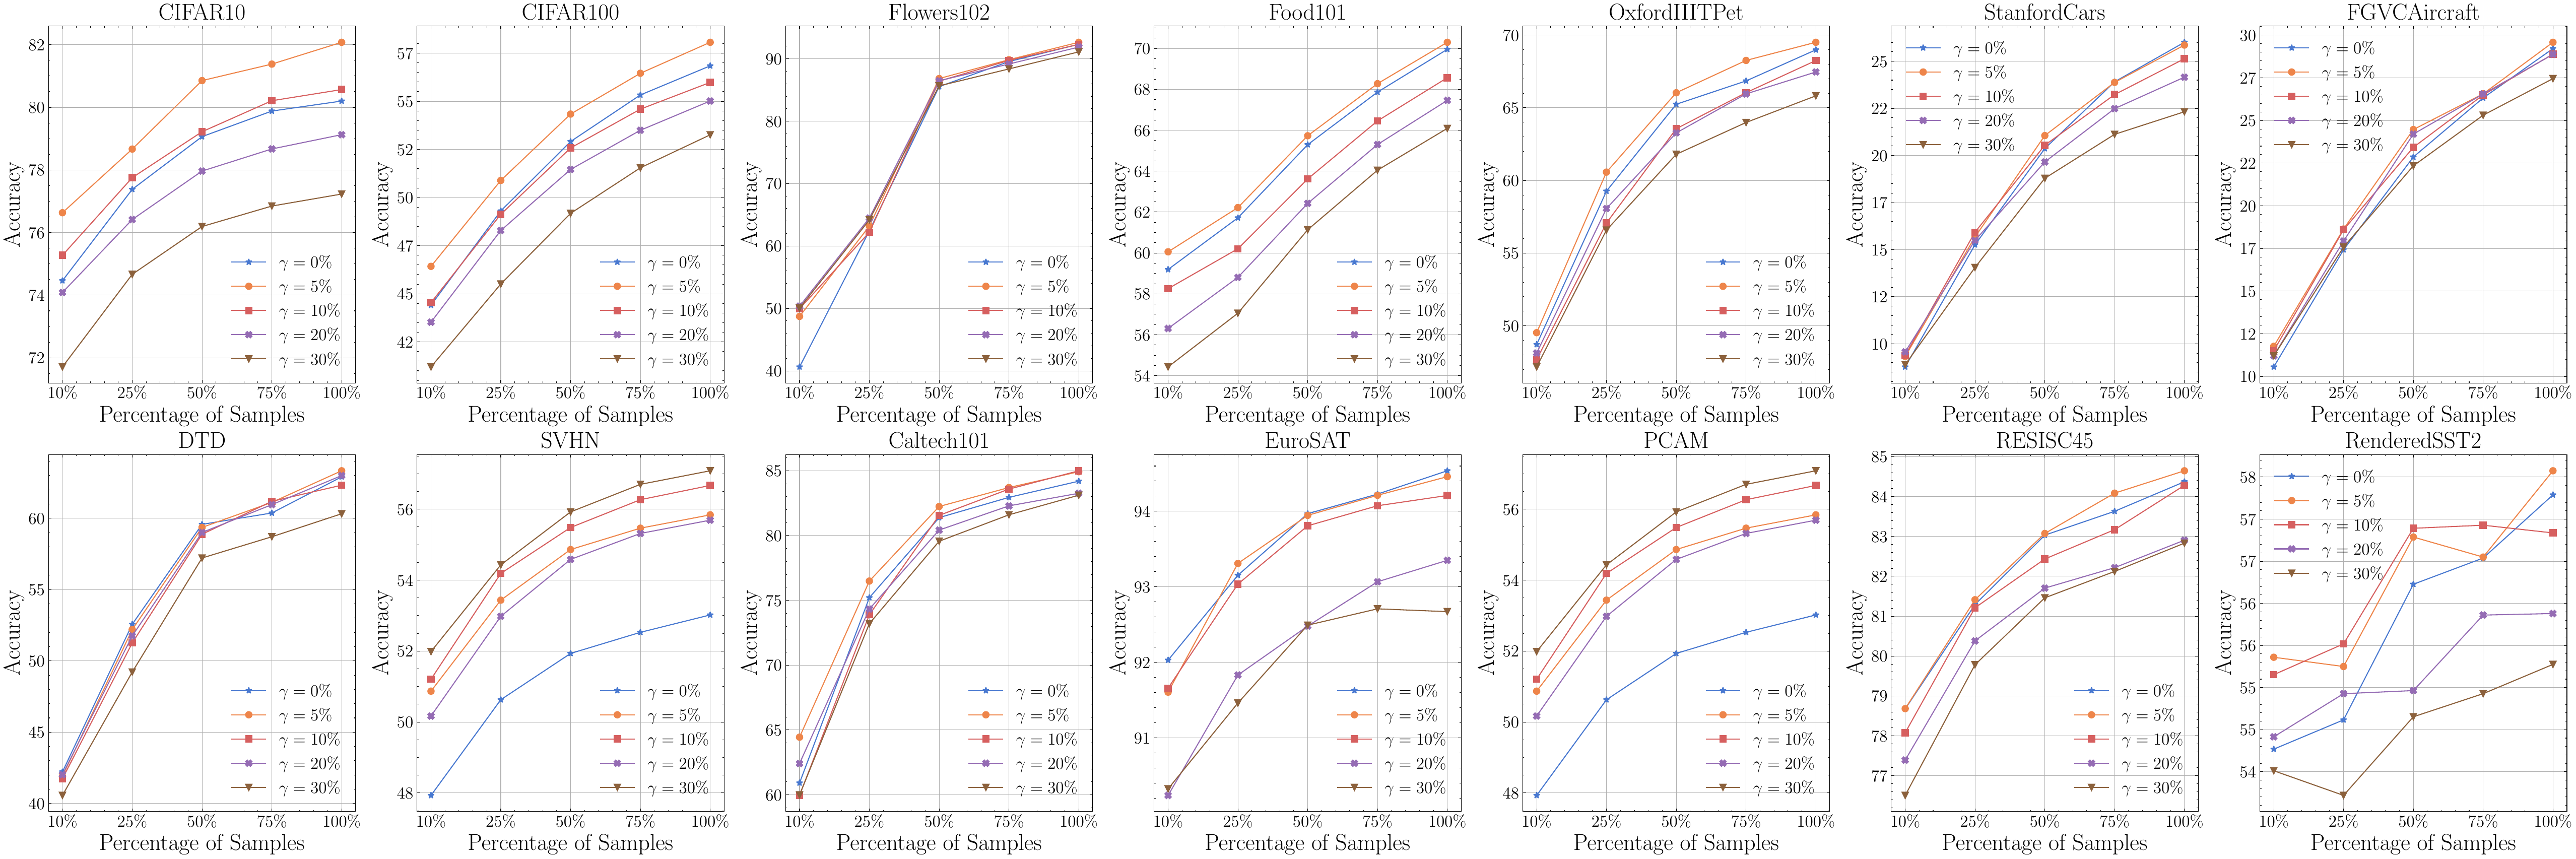}
    \caption{YFCC15M pre-trained ResNet-50 in-domain (ID) evaluation results}
    \label{fig:append-yfcc15m-r50-id-eval}
\end{figure}

\begin{figure}[h]
    \centering
    \includegraphics[width=0.85\textwidth]{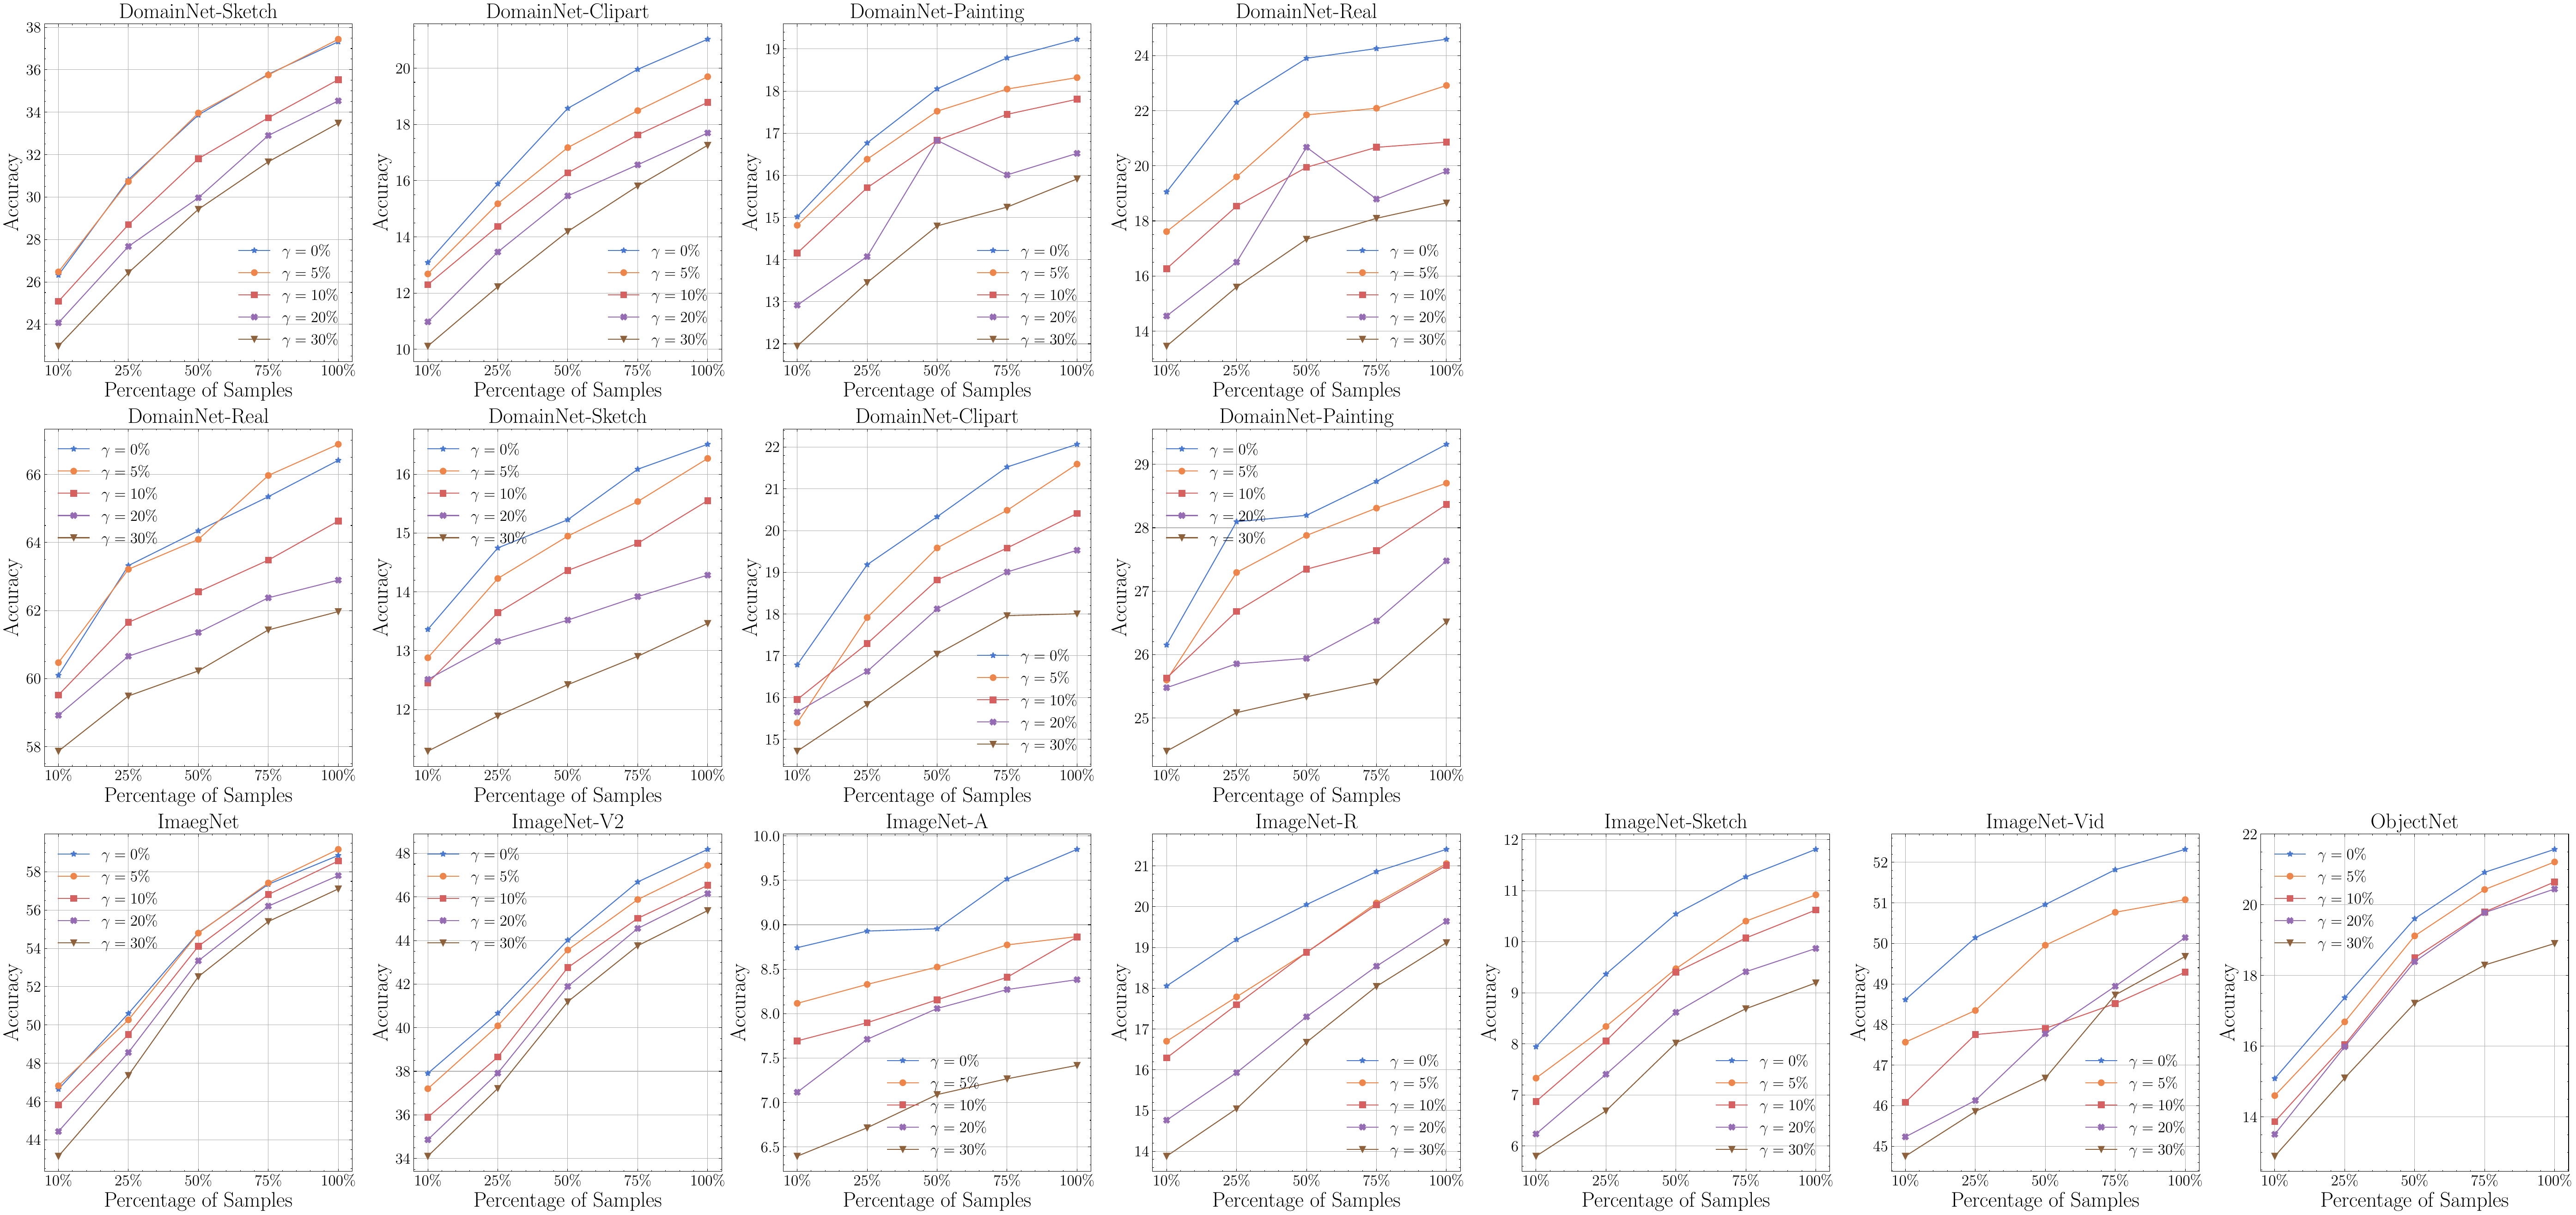}
    \caption{YFCC15M pre-trained ResNet-50 out-of-domain (OOD) evaluation results}
    \label{fig:append-yfcc15m-r50-odd-eval}
\end{figure}

\subsection{Detailed ID and OOD Singular Value Spectrum}
\label{sec:append-id-ood-svd}

We plot the singular value spectrum for ID datasets and OOD datasets of the noisy ResNet-50 models. 
To better visualize the spectrum, we split the singular values into three groups: the top 20, 20-500, and the remaining. 

The singular value spectrum of the ID datasets is shown in \cref{fig:append-in1k-r50-id-svd} and \cref{fig:append-yfcc15m-r50-id-svd} respectively. From 20-500 singular values visualization, we can observe that the noisy pre-trained models in general have larger singular values in this range, corresponding to a feature space that spans more of its coordinates. We summarize this visualization as the SVE introduced \cref{sec:understand}. 
\revision{
Here, we provide more explanation how to make \cref{fig:r50_id_ood_svd}. First, each color and marker represents a different pre-training noise ratio. We plot the average accuracy of different percentage of downstream datasets and the SVD (or LSVR) of the downstream test data for each downstream task. Thus each points corresponds to a downstream task. The results of different pre-training noise ratio for each task are thus clustered together. }

\revision{
We also provide a zoom-in version for \cref{fig:r50_in1k_id_svd} and \cref{fig:r50_in1k_ood_svd} for better visualization, as shown in \cref{fig:r50_id_ood_svd_zoomin}.
}

\begin{figure}[!t]
\centering
    \hfill
    \subfigure[\revision{IN1K, ID}]{\label{fig:r50_in1k_id_svd_zoomin}\includegraphics[width=0.48\linewidth]{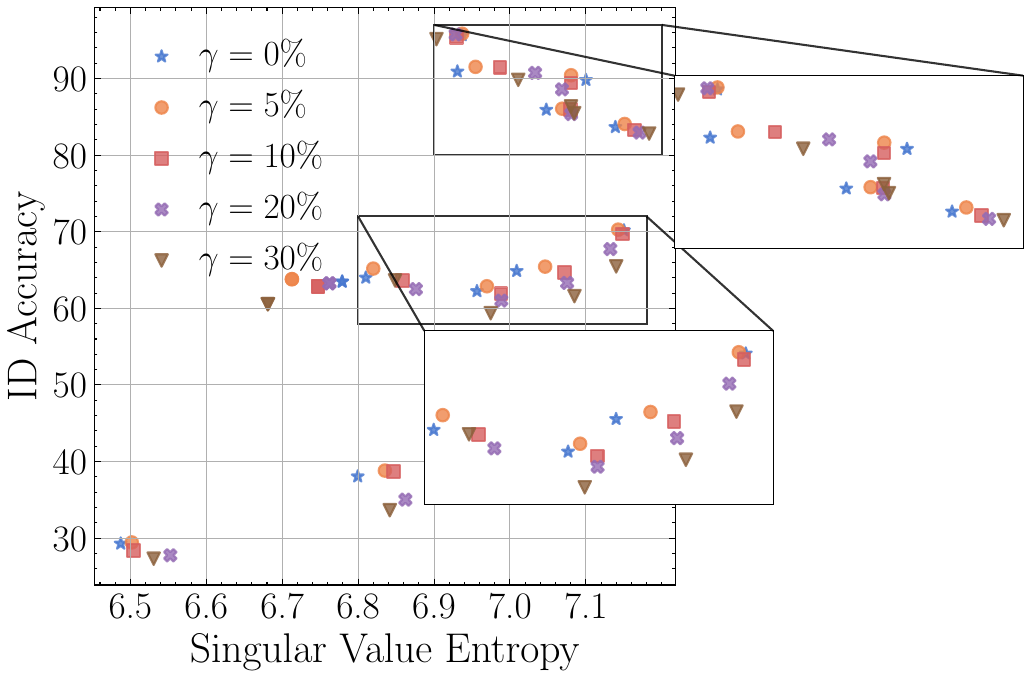}}
    \hfill
    \subfigure[\revision{YFCC15M, ID}]{\label{fig:r50_in1k_ood_svd_zoomin}\includegraphics[width=0.48\linewidth]{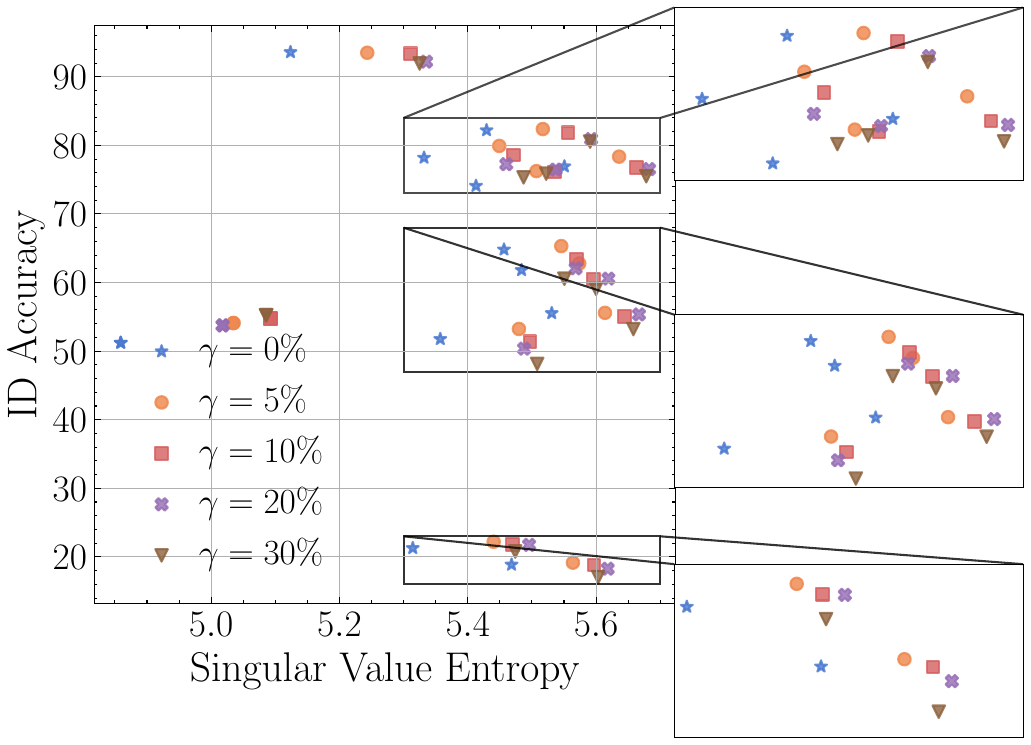}}
    \hfill
\caption{
\revision{Zoom-in visualization of feature SVE analysis for in-domain (ID) tasks. }
% Feature SVD analysis. We compute the singular value entropy (SVE) for in-domain (ID) tasks and the largest singular value ratio (LSVR) for out-of-domain (OOD) tasks. Both metrics are computed for ImageNet-1K fully supervised pre-trained ((a) and (b)) and YFCC15M CLIP pre-trained ((c) and (d)) models. The SVE first slightly improves as the noise ratio increases to $5\%$ or $10\%$, indicating better generalization. As the noise ratio increases, the SVE further improves, and the LSVR drops significantly, corresponding to worse generalization on ID and OOD tasks, as more noise structure is learned. The dominant singular components become less transferable. 
% \wjd{Move the legend of 3(a) elsewhere? Seems the legend mixes with the plot.}
% \ank{Can we make the legend and the text bold as when the pdf is at size of A4 sheet - the figures are difficult to read}
} 
\label{fig:r50_id_ood_svd_zoomin}
\end{figure}

The singular value spectrum of the OOD datasets is shown in \cref{fig:append-in1k-r50-odd-svd} and \cref{fig:append-yfcc15m-r50-odd-svd} respectively. From the top 20 singular values visualization, we can observe that the clean pre-trained model tends to present larger singular values in this range, especially the largest singular value. 
We connect this observation with the transferability performance on OOD tasks \citep{chen19itrans}, and summarize it as LSVR introduced in \cref{sec:understand}. 

\begin{figure}
    \centering
    \includegraphics[width=0.85\textwidth]{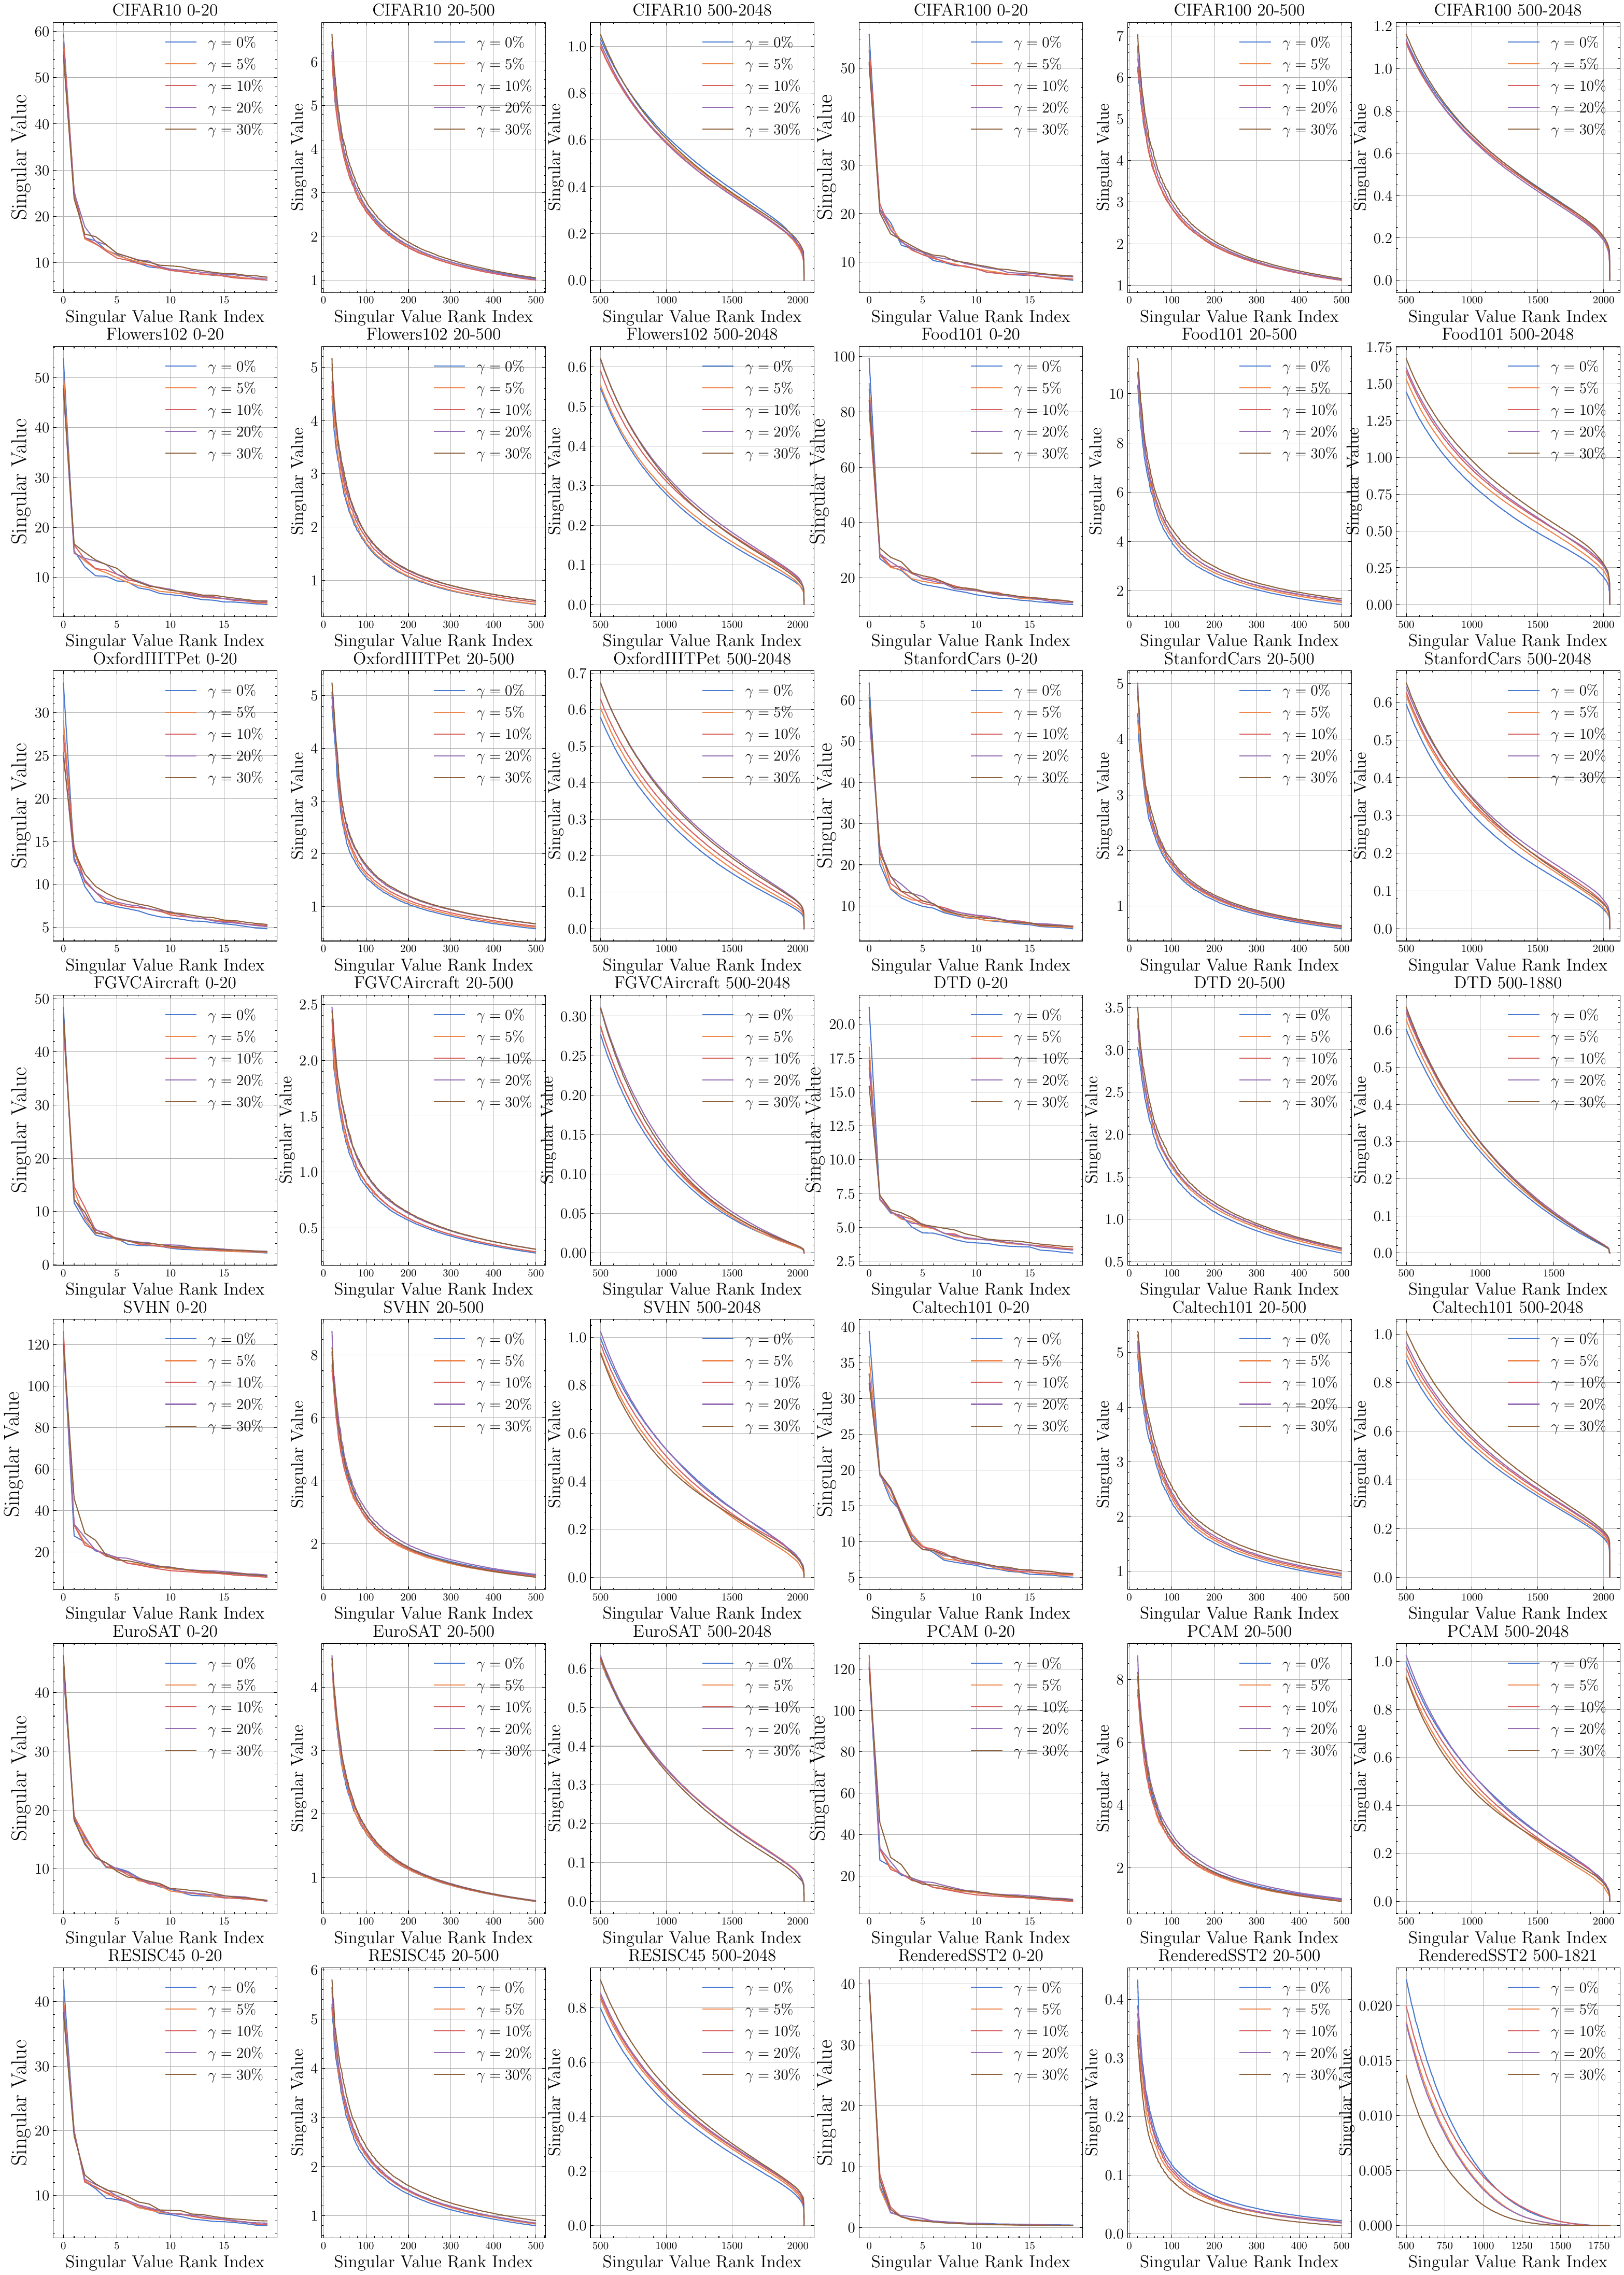}
    \caption{ImageNet-1K R50 in-domain (ID) feature SVD spectrum analysis}
    \label{fig:append-in1k-r50-id-svd}
\end{figure}

\begin{figure}
    \centering
    \includegraphics[width=0.85\textwidth]{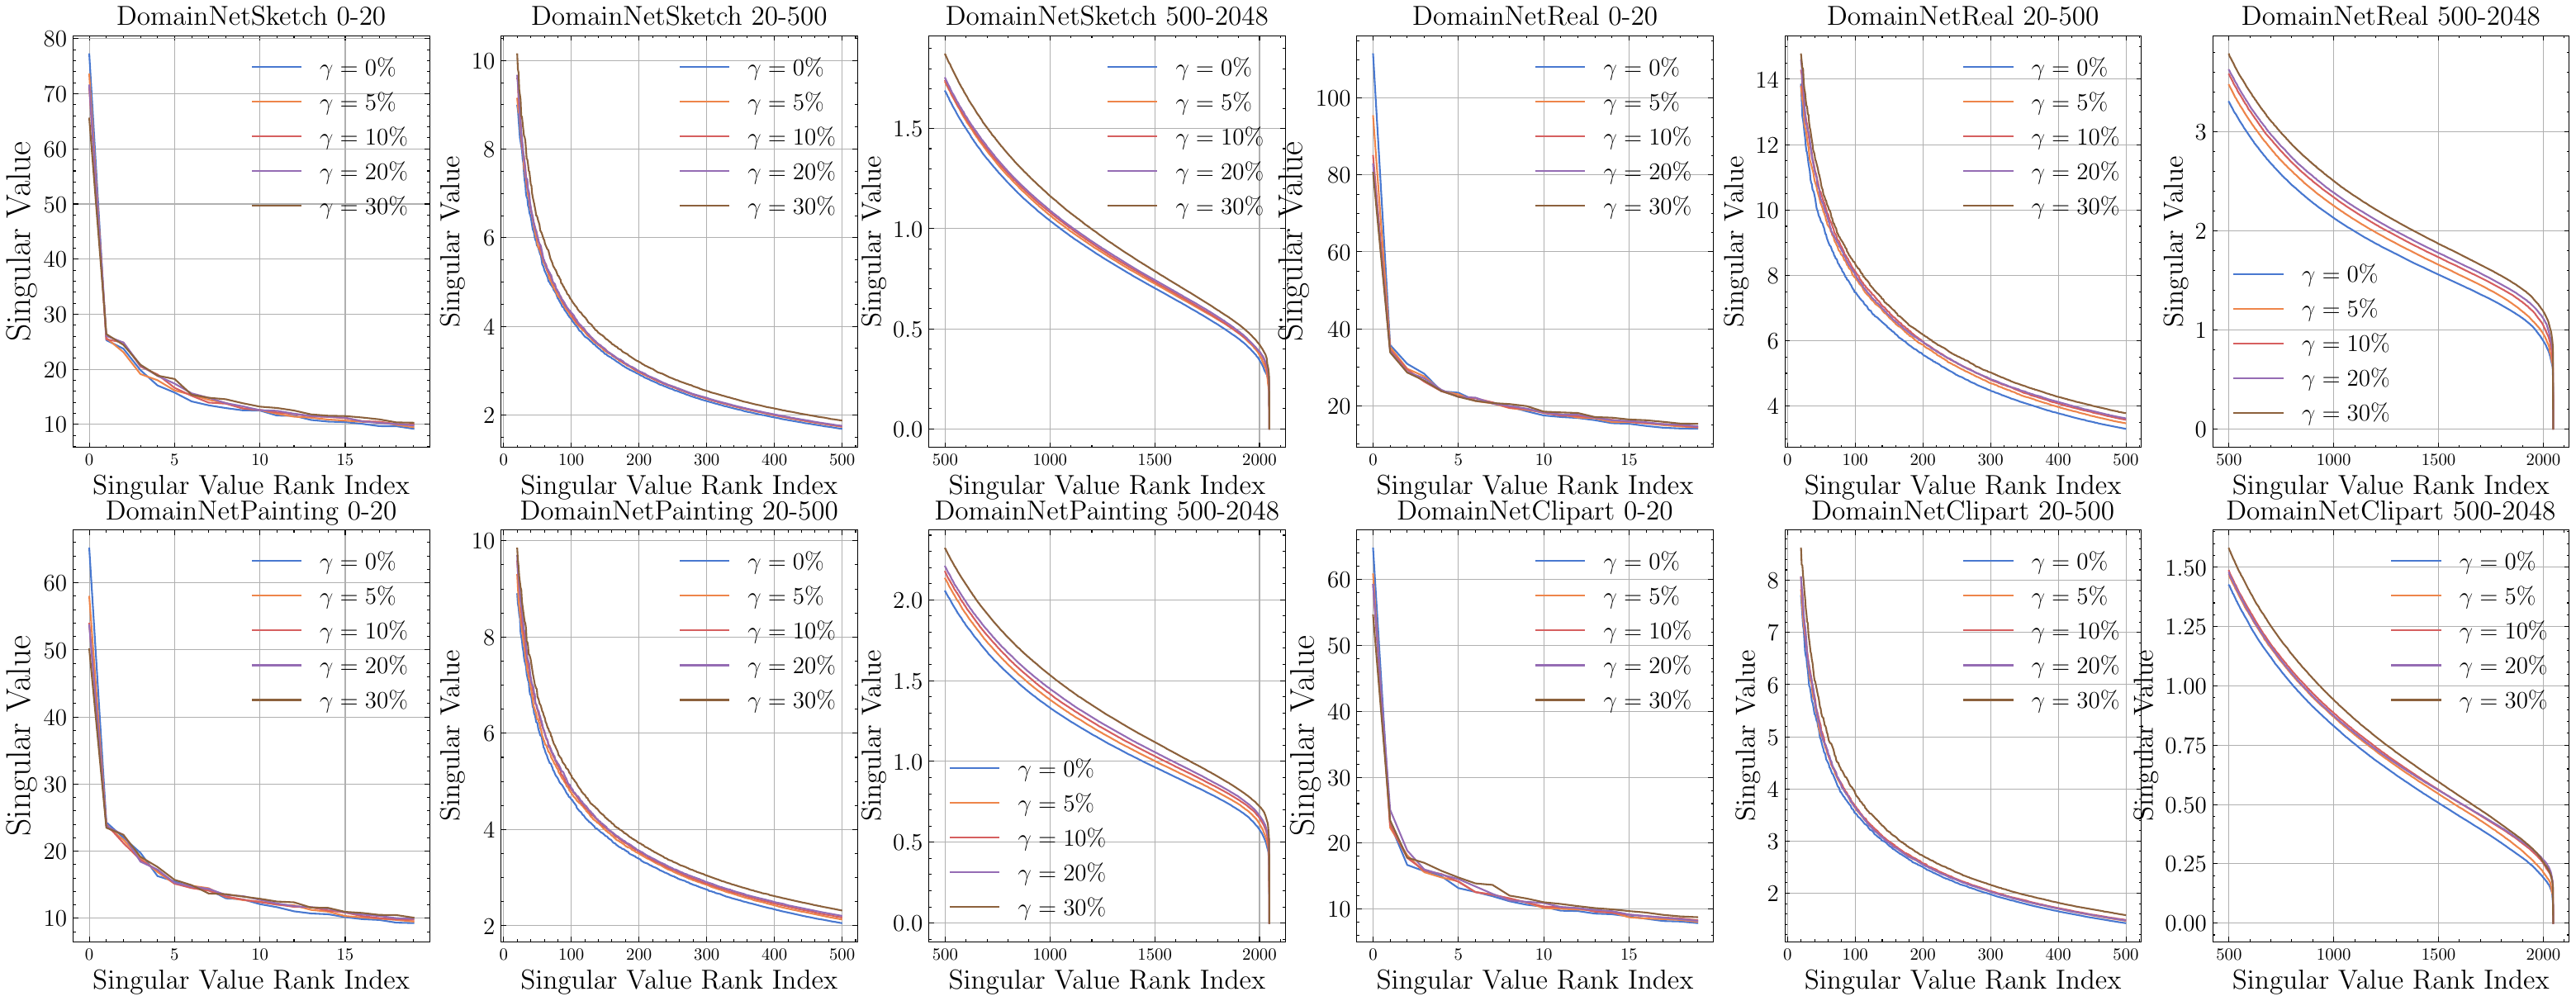}
    \caption{ImageNet-1K R50 out-of-domain (OOD) feature SVD spectrum analysis}
    \label{fig:append-in1k-r50-odd-svd}
\end{figure}

\begin{figure}
    \centering
    \includegraphics[width=0.85\textwidth]{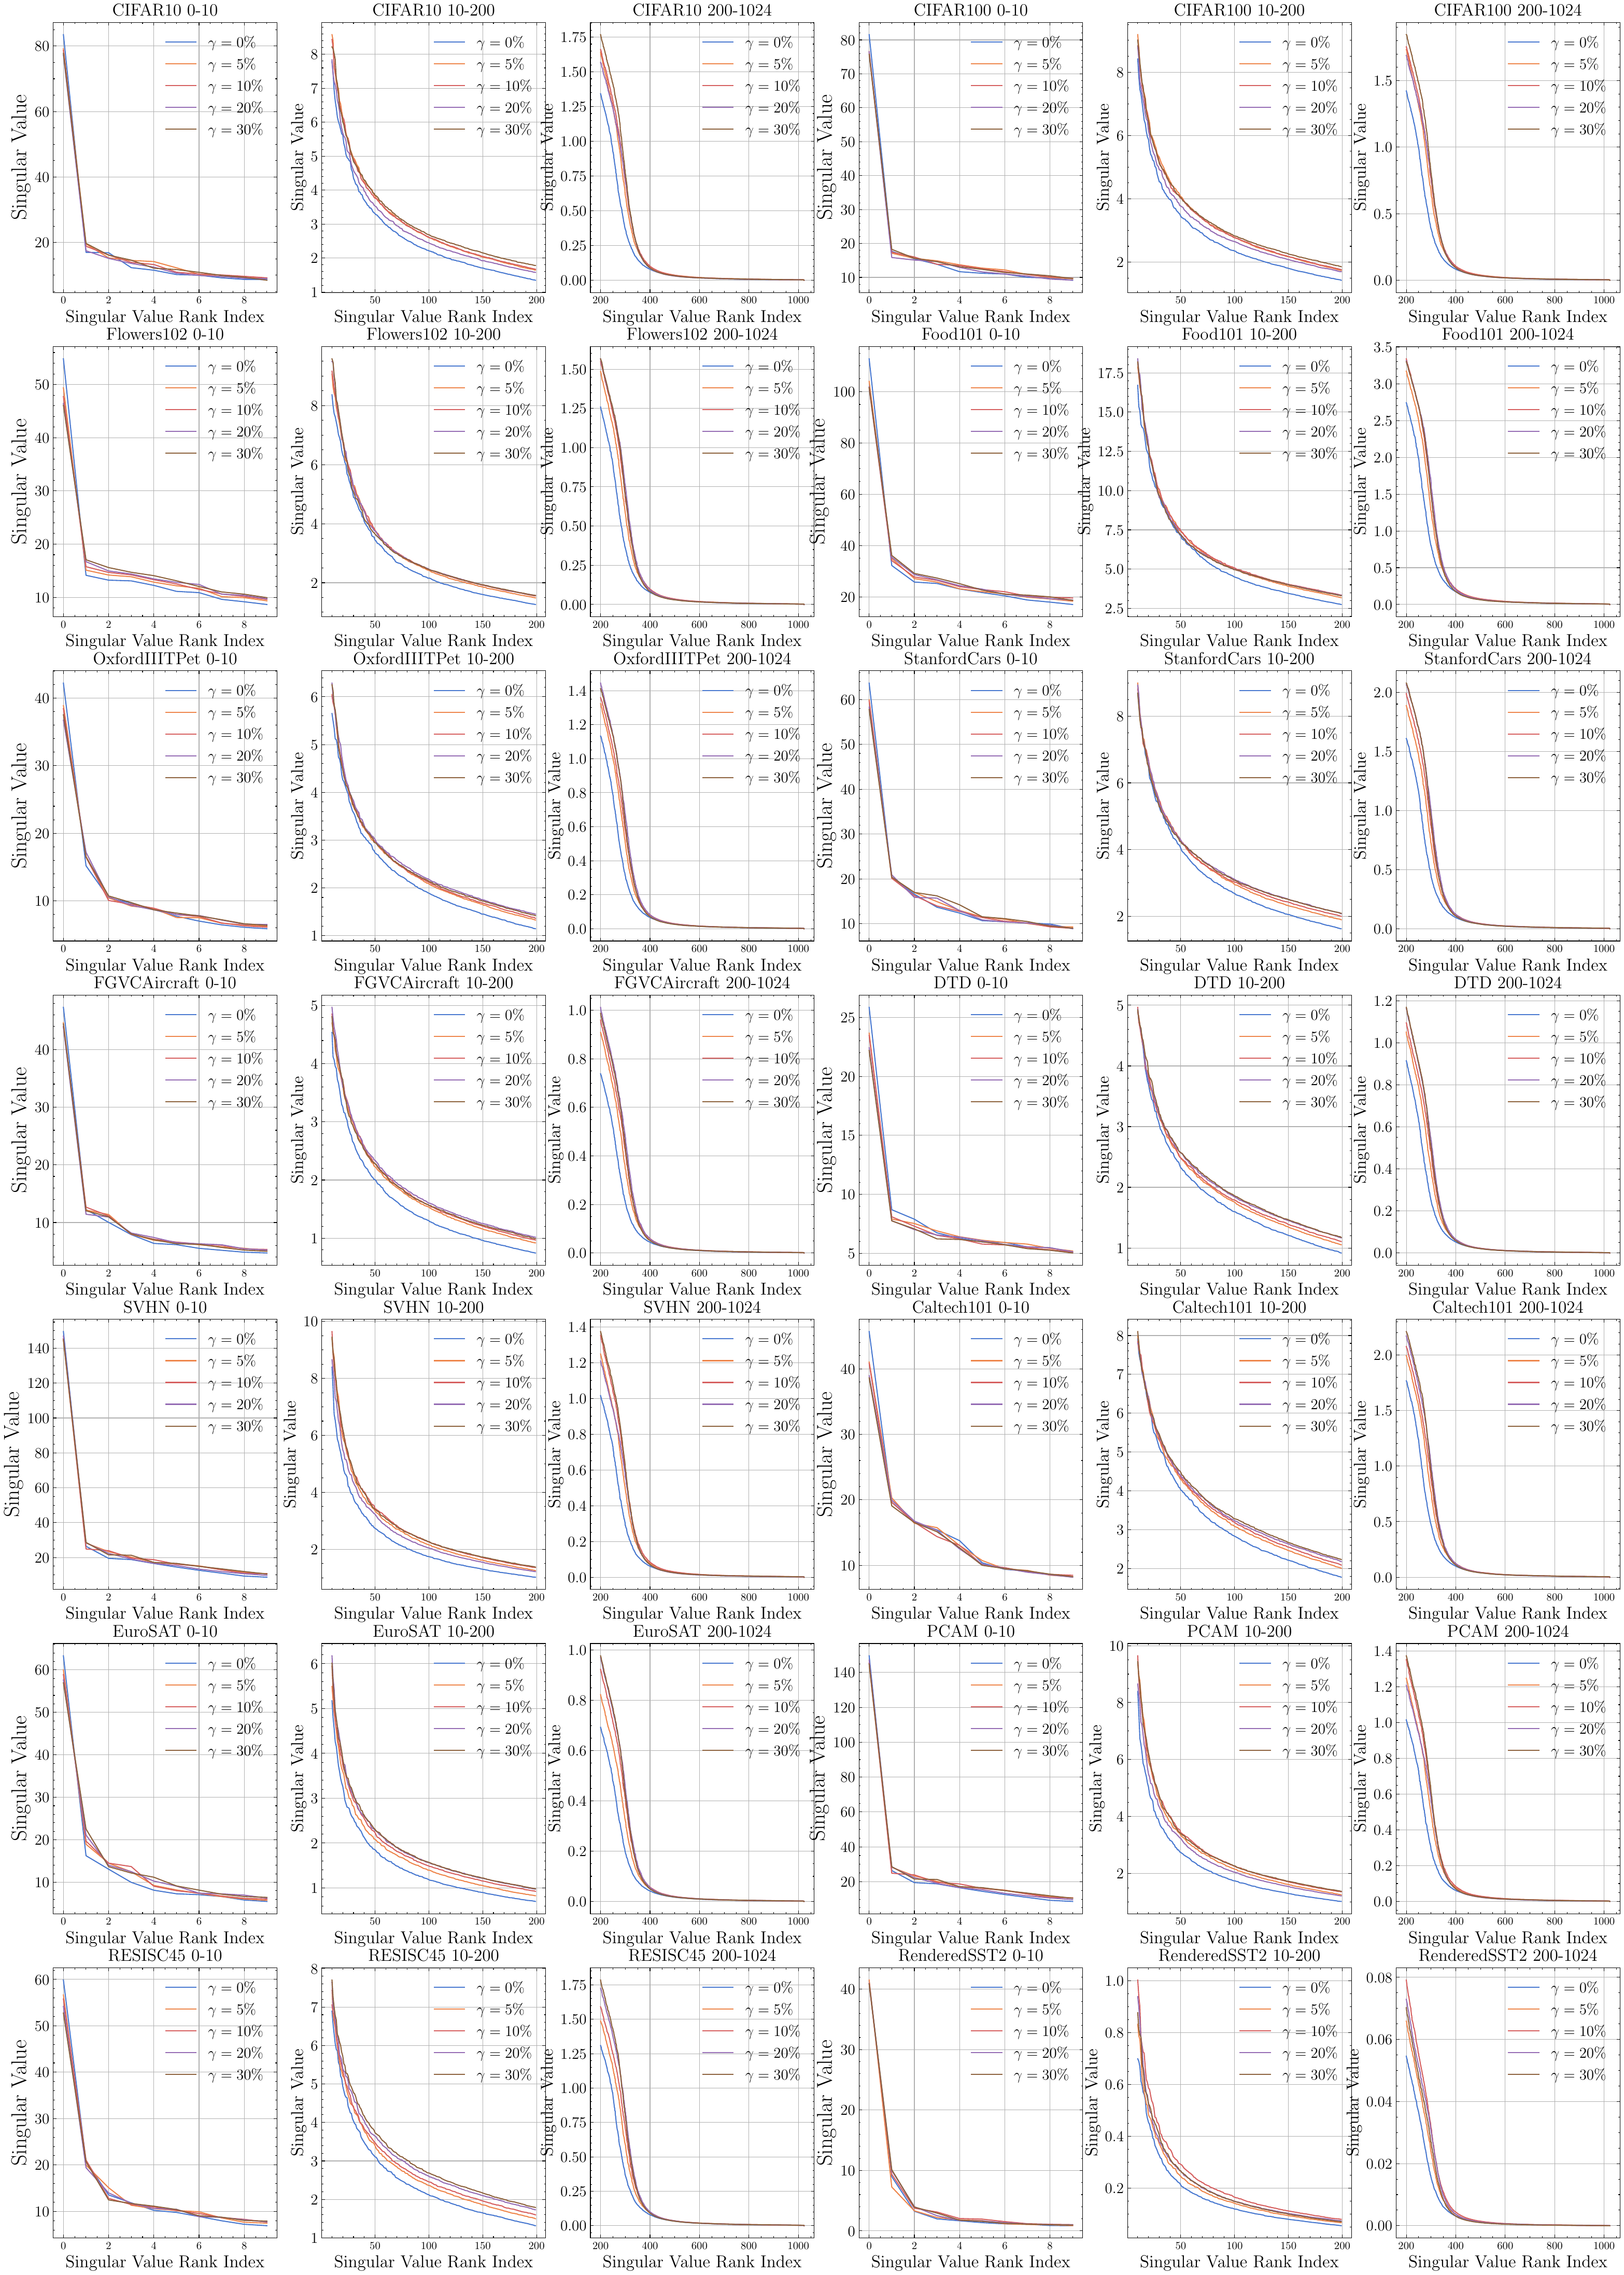}
    \caption{YFCC15M R50 in-domain (ID) feature SVD spectrum analysis}
    \label{fig:append-yfcc15m-r50-id-svd}
\end{figure}

\begin{figure}
    \centering
    \includegraphics[width=0.85\textwidth]{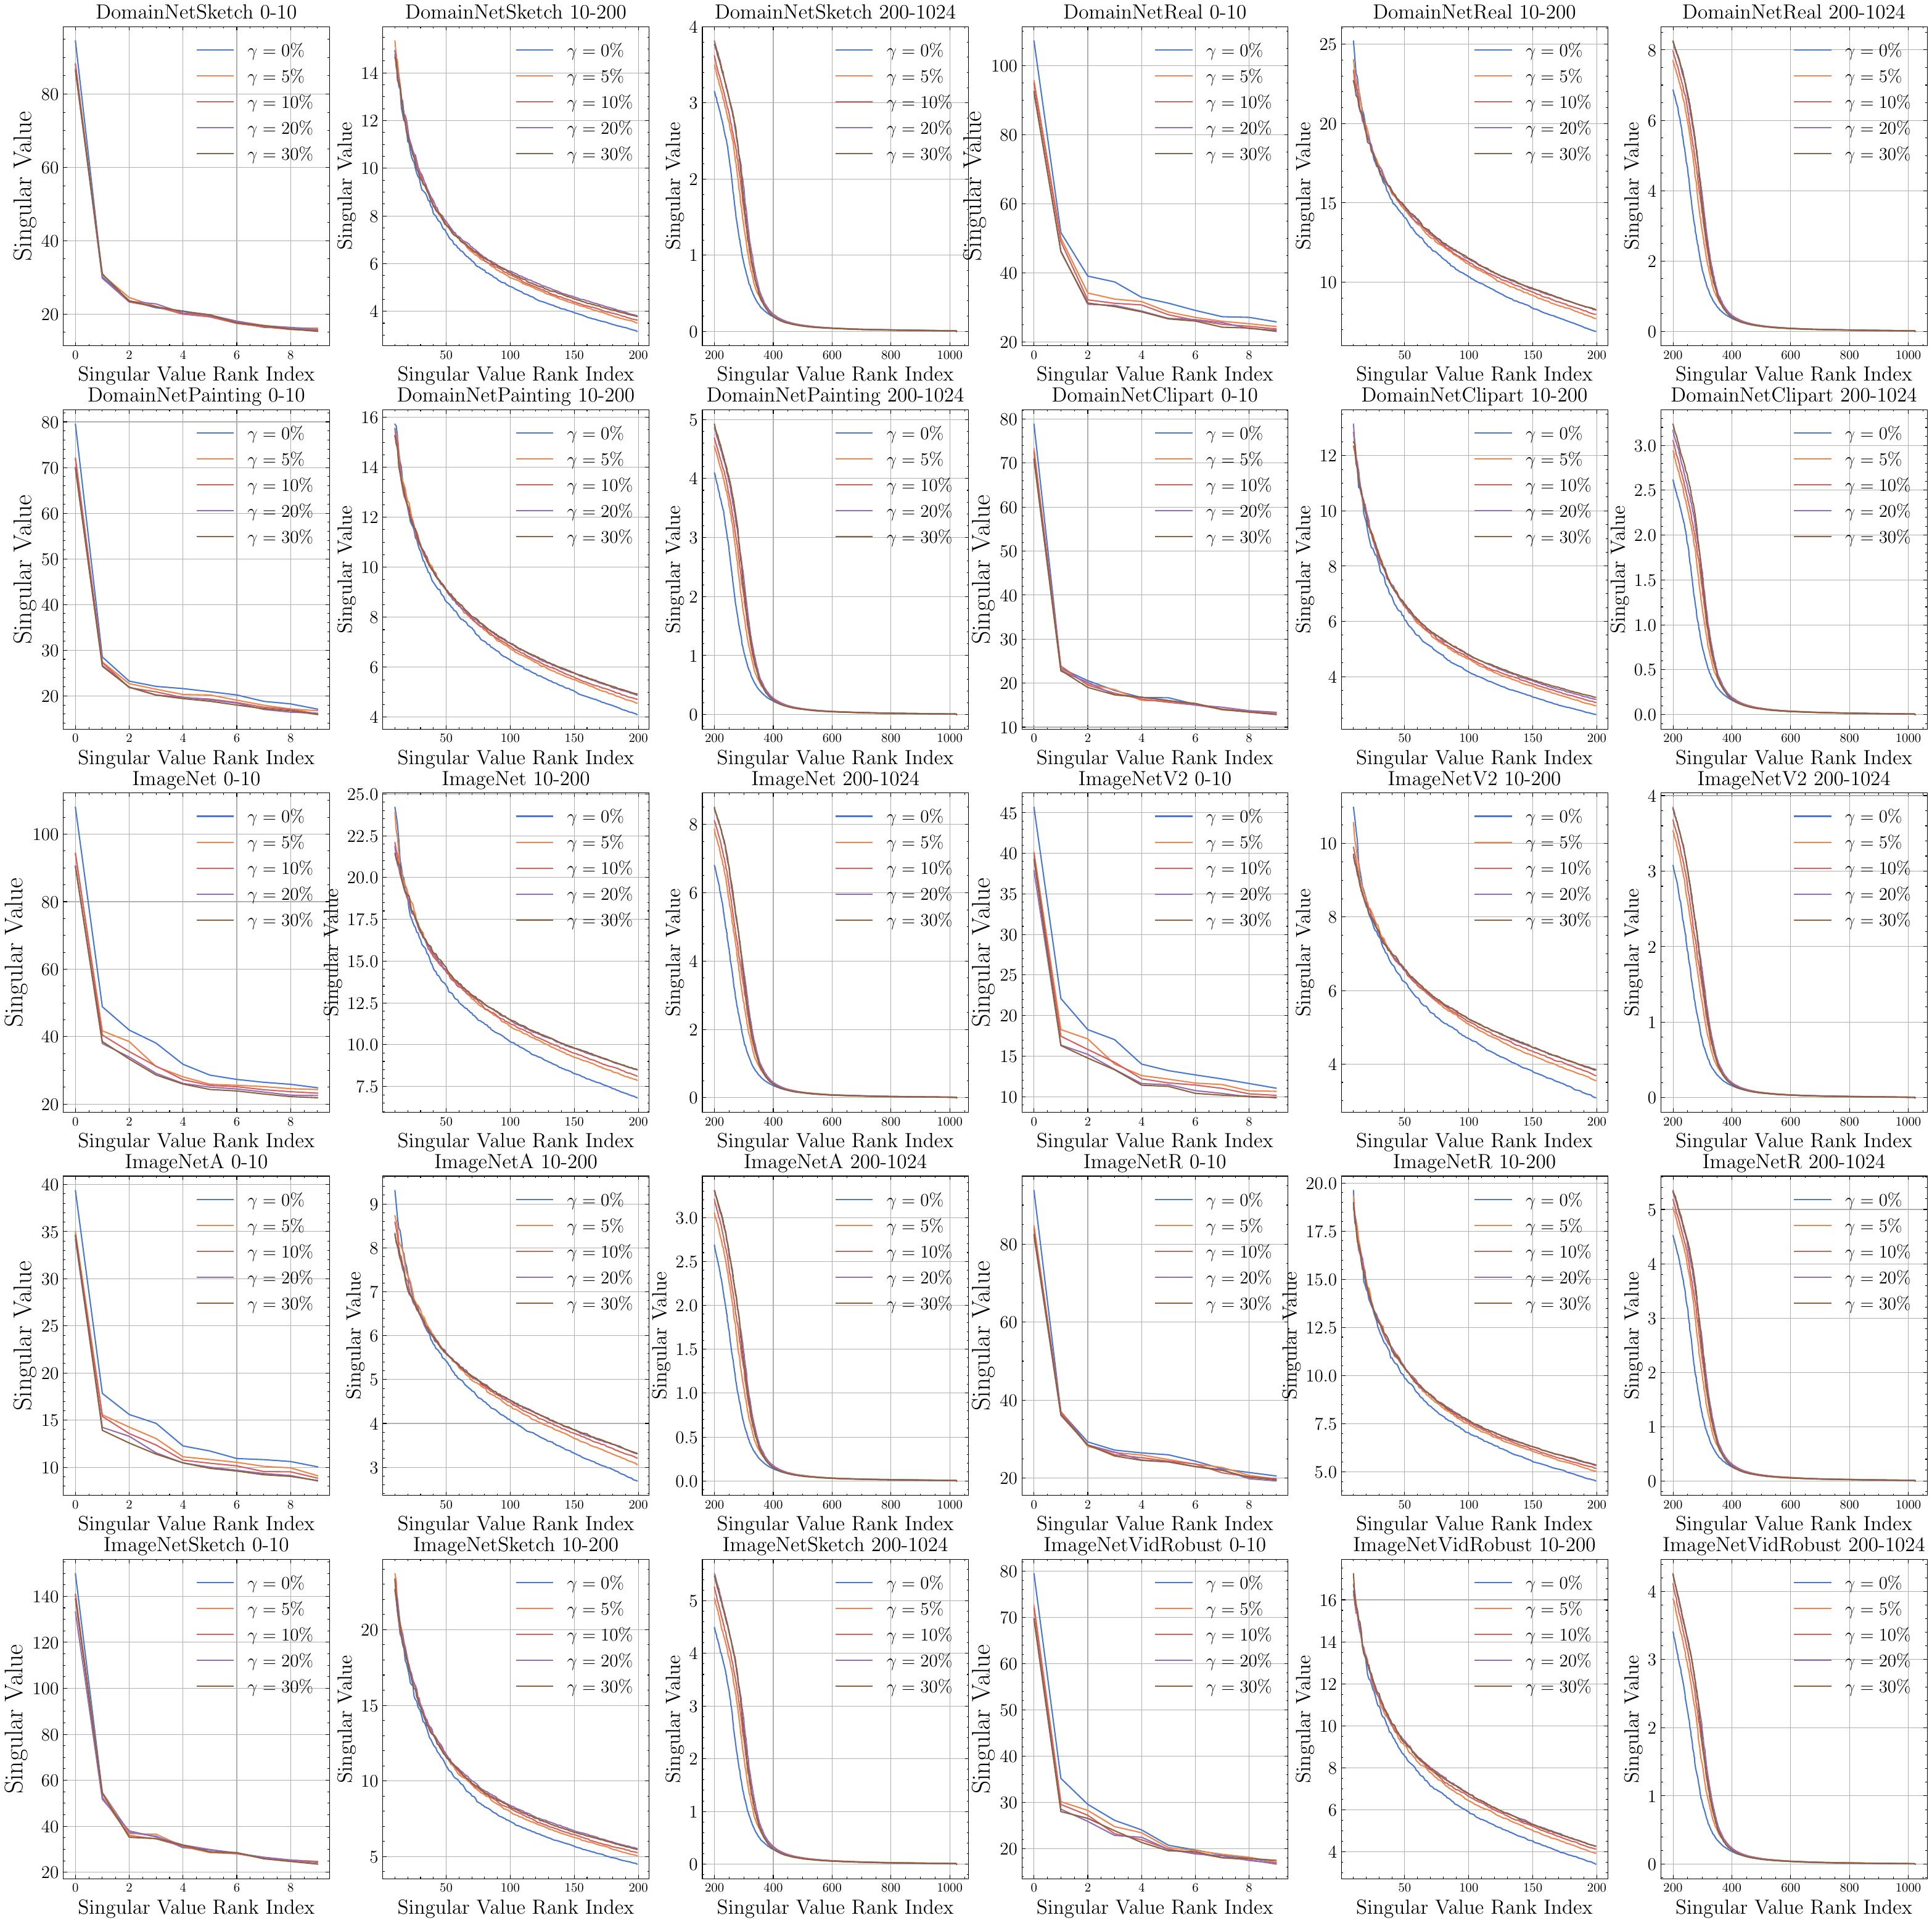}
    \caption{YFCC15M R50 out-of-domain (OOD) feature SVD spectrum analysis}
    \label{fig:append-yfcc15m-r50-odd-svd}
\end{figure}

\section{Experiments}
\label{sec:append-exp}

More details of experiments in \cref{sec-exp} are shown here.

% \subsection{}
% \label{sec:append-exp-vision}

\subsection{Detailed Setup for Vision Models Experiments}
\label{sec:append-exp-vision-setup}

We provide a more detailed setup of evaluation on practical vision models. 
First, we summarize the noisy pre-trained models with their pre-trained dataset, parameter size, and validation accuracy on ImageNet-1K we used in \cref{tab:vision-model-details}.
We use the same ID vision and OOD vision datasets as in \cref{tab:append-exp-vision-id} and \cref{tab:append-exp-vision-odd} for evaluation.
Each experiment is run with three random seeds. 

\begin{table}[h]
\centering
\caption{Noisy vision models we evaluated.}
\label{tab:vision-model-details}
\resizebox{\textwidth}{!}{%
\begin{tabular}{@{}cccc@{}}
\toprule
Model & Pre-trained Data & Pre-trained Method & Param. Size (M) \\ \midrule
EfficientNet-B3 \citep{tan2019efficientnet}      &    JFT-300M \citep{hinton2015distilling}             &      Noisy Student \citep{xie2020ns}          &          12.23      \\
ResNetv2-152x2 \citep{he2016identity}      &          ImageNet-21K   \citep{ridnik2021imagenet21k}     &                  BiT \cite{kolesnikov2020big}    &        236.34  \\ 
Swin-L \citep{liu2021swin}      &          ImageNet-21K   \citep{ridnik2021imagenet21k}         &           Supervised \citep{liu2021swin}         &        196.74    \\ 
ViT-L \citep{dosovitskiy2020image}      &         Laion-2B    \citep{schuhmann2022laionb}     &         CLIP  \citep{radford2021learning}            &    304.20      \\ 
ConvNext-L \citep{liu2022convnext}      &            Laion-2B   \citep{schuhmann2022laionb}         &           CLIP  \citep{radford2021learning}           &   200.13      \\ 
\bottomrule
\end{tabular}%
}
\end{table}

We mainly compare our method with MLP tuning and LP, where we fine-tuning the modules using AdamW \citep{kingma2014adam} for $30$ epochs with a cosine learning rate scheduler. We set the learning rate as $0.1$ and weight decay of $0$ for LP, and set the learning rate as $0.001$ and weight decay of $1$e$-4$ for MLP tuning and our method.

\subsection{Detailed Results for Vision Models Experiments}
\label{sec:append-exp-vision-res}

More results on each evaluated dataset are provided here. The ID results with standard deviation in accuracy on each ID datasets are shown in \cref{tab:res-cv-id}, and the OOD results with standard deviation in accuracy on the evaluated OOD datasets are shown in \cref{tab:res-cv-ood}.
% For ID results, we additionally compare with a recent black-box tuning work - BlackVIP \citep{oh2023blackvip}. It is designed for vision transformers and thus we compare it with NMTune on Laion-2B pre-trained ViT-L. 
% The partial results we obtained for BlackVIP show that its performance is singificantly

\begin{table}[h]
\centering
\caption{Evaluation of our method on vision models in practice that are pre-trained on noisy datasets. We compare different methods on 14 vision datasets for in-domain (ID) evaluation}
\label{tab:res-cv-id}
\resizebox{\textwidth}{!}{%
\begin{tabular}{@{}l|l|cccccccccccccc|c@{}}
\toprule
\multicolumn{1}{c|}{\begin{tabular}[c]{@{}c@{}}Pre-trained \\ Model\end{tabular}} &
  \multicolumn{1}{c|}{\begin{tabular}[c]{@{}c@{}}Tuning\\ Method\end{tabular}} &
  CIFAR10 &
  CIFAR100 &
  Flowers102 &
  Food101 &
  OxfordIIITPet &
  StanfordCars &
  FGVCAircraft &
  DTD &
  SVHN &
  Caltech101 &
  EuroSAT &
  PCAM &
  RESISC45 &
  RenderedSST2 &
  Avg \\  \midrule
\multirow{3}{*}{\begin{tabular}[c]{@{}l@{}}JFT-300M \\ Semi-Supervised\\ EfficientNet-B3\end{tabular}} &
  LP &
  94.68$\pm$0.12 &
  79.00$\pm$0.23 &
  91.43$\pm$0.09 &
  79.71$\pm$1.02 &
  94.92$\pm$0.11 &
  59.36$\pm$0.98 &
  43.82$\pm$1.34 &
  73.60$\pm$0.20 &
  63.77$\pm$0.99 &
  \textbf{90.65$\pm$0.32} &
  95.88$\pm$0.01 &
  63.77$\pm$1.44 &
  89.62$\pm$0.87 &
  \textbf{53.93$\pm$0.23} &
  76.72 \\
 &
  MLP &
  95.87$\pm$0.08 &
  79.51$\pm$0.14 &
  87.78$\pm$0.53 &
  82.26$\pm$0.54 &
  94.96$\pm$0.11 &
  57.70$\pm$0.74 &
  41.46$\pm$2.42 &
  72.55$\pm$0.21 &
  \textbf{67.19$\pm$1.28} &
  87.52$\pm$0.58 &
  97.10$\pm$0.02 &
  \textbf{67.19$\pm$0.98} &
  92.25$\pm$0.54 &
  52.85$\pm$0.18 &
  76.87 \\
 &
  Ours &
  \textbf{96.15$\pm$0.05} &
  \textbf{79.71$\pm$0.10} &
  \textbf{91.61$\pm$0.09} &
  \textbf{82.63$\pm$0.51} &
  \textbf{95.29$\pm$0.13} &
  \textbf{60.24$\pm$0.69} &
  \textbf{43.57$\pm$1.02} &
  \textbf{73.78$\pm$0.18} &
  67.05$\pm$0.54 &
  88.73$\pm$0.44 &
  \textbf{97.20$\pm$0.01} &
  67.05$\pm$0.91 &
  \textbf{92.60$\pm$0.40} &
  51.25$\pm$0.08 &
  \textbf{77.63} \\  \midrule
\multirow{3}{*}{\begin{tabular}[c]{@{}l@{}}ImageNet-21K\\ Fully Supervised\\ ResNetv2-152x2\end{tabular}} &
  LP &
  96.39$\pm$0.13 &
  85.21$\pm$0.17 &
  96.85$\pm$0.08 &
  85.99$\pm$0.47 &
  91.73$\pm$0.20 &
  55.96$\pm$1.23 &
  43.37$\pm$0.98 &
  73.51$\pm$0.55 &
  62.51$\pm$0.83 &
  \textbf{92.15$\pm$0.16} &
  97.15$\pm$0.13 &
  58.70$\pm$0.87 &
  92.20$\pm$0.43 &
  53.47$\pm$0.32 &
  77.51 \\
 &
  MLP &
  97.02$\pm$0.11 &
  85.47$\pm$0.19 &
  96.96$\pm$0.09 &
  \textbf{86.46$\pm$0.34} &
  92.39$\pm$0.23 &
  57.25$\pm$1.12 &
  41.10$\pm$1.45 &
  73.76$\pm$0.43 &
  64.61$\pm$0.56 &
  89.50$\pm$0.21 &
  97.59$\pm$0.11 &
  59.66$\pm$0.45 &
  93.33$\pm$0.27 &
  51.02$\pm$0.59 &
  77.58 \\
 &
  Ours &
  \textbf{97.12$\pm$0.11} &
  \textbf{85.68$\pm$0.16} &
  \textbf{96.98$\pm$0.08} &
  85.69$\pm$0.35 &
  \textbf{92.49$\pm$0.18} &
  \textbf{57.42$\pm$0.99} &
  \textbf{43.54$\pm$1.23} &
  \textbf{73.87$\pm$0.46} &
  \textbf{66.94$\pm$0.50} &
  92.01$\pm$0.12 &
  \textbf{97.67$\pm$0.09} &
  \textbf{61.12$\pm$0.41} &
  \textbf{93.97$\pm$0.35} &
  \textbf{53.53$\pm$0.71} &
  \textbf{78.43} \\  \midrule
\multirow{3}{*}{\begin{tabular}[c]{@{}l@{}}ImageNet-21K\\ Fully Supervised\\ Swin-L\end{tabular}} &
  LP &
  98.06$\pm$0.07 &
  88.51$\pm$0.12 &
  99.27$\pm$0.04 &
  89.68$\pm$0.63 &
  92.60$\pm$0.19 &
  65.43$\pm$0.34 &
  53.48$\pm$1.44 &
  77.45$\pm$0.39 &
  72.94$\pm$0.33 &
  \textbf{90.91$\pm$0.09} &
  97.00$\pm$0.50 &
  72.94$\pm$0.23 &
  93.84$\pm$0.21 &
  54.59$\pm$0.70 &
  81.91 \\
 &
  MLP &
  98.45$\pm$0.06 &
  89.72$\pm$0.09 &
  99.12$\pm$0.05 &
  91.20$\pm$0.30 &
  93.75$\pm$0.24 &
  68.15$\pm$1.22 &
  52.81$\pm$0.78 &
  77.63$\pm$0.42 &
  73.48$\pm$0.32 &
  89.26$\pm$0.22 &
  \textbf{98.07$\pm$0.10} &
  74.48$\pm$0.37 &
  95.04$\pm$0.23 &
  54.09$\pm$0.52 &
  82.52 \\
 &
  Ours &
  \textbf{98.60$\pm$0.06} &
  \textbf{90.14$\pm$0.11} &
  \textbf{99.53$\pm$0.03} &
  \textbf{91.40$\pm$0.33} &
  \textbf{94.22$\pm$0.22} &
  \textbf{75.60$\pm$2.12} &
  \textbf{55.95$\pm$0.91} &
  \textbf{79.97$\pm$0.20} &
  \textbf{76.61$\pm$0.12} &
  90.36$\pm$0.26 &
  98.06$\pm$0.11 &
  \textbf{76.61$\pm$0.41} &
  \textbf{95.34$\pm$0.23} &
  \textbf{55.92$\pm$0.48} &
  \textbf{84.17} \\  \midrule
\multirow{3}{*}{\begin{tabular}[c]{@{}l@{}}Laion-2B\\ CLIP\\ ConvNext-L\end{tabular}} &
  LP &
  98.15$\pm$0.08 &
  88.83$\pm$0.24 &
  \textbf{98.72$\pm$0.12} &
  91.68$\pm$0.28 &
  94.07$\pm$0.15 &
  94.68$\pm$0.33 &
  65.94$\pm$0.45 &
  \textbf{83.88$\pm$0.04} &
  82.41$\pm$0.21 &
  \textbf{96.37$\pm$0.03} &
  97.78$\pm$0.01 &
  82.41$\pm$0.21 &
  95.44$\pm$0.05 &
  73.70$\pm$0.10 &
  88.86 \\
 &
  MLP &
  98.64$\pm$0.05 &
  89.67$\pm$0.18 &
  96.35$\pm$0.47 &
  92.80$\pm$0.41 &
  93.55$\pm$0.13 &
  94.47$\pm$0.32 &
  67.06$\pm$0.75 &
  81.33$\pm$0.24 &
  82.08$\pm$0.45 &
  94.33$\pm$0.02 &
  98.22$\pm$0.03 &
  82.25$\pm$0.15 &
  96.51$\pm$0.14 &
  72.27$\pm$0.14 &
  88.54 \\
 &
  Ours &
  \textbf{98.73$\pm$0.06} &
  \textbf{90.39$\pm$0.14} &
  98.50$\pm$0.26 &
  \textbf{92.90$\pm$0.24} &
  \textbf{94.52$\pm$0.12} &
  \textbf{95.48$\pm$0.19} &
  \textbf{69.18$\pm$0.51} &
  83.23$\pm$0.19 &
  \textbf{82.83$\pm$0.17} &
  95.26$\pm$0.05 &
  \textbf{98.46$\pm$0.03} &
  \textbf{82.53$\pm$0.15} &
  \textbf{96.82$\pm$0.08} &
  \textbf{73.94$\pm$0.23} &
  \textbf{89.48} \\  \midrule
\multirow{3}{*}{\begin{tabular}[c]{@{}l@{}}Laion-2B\\ CLIP\\ ViT-L\end{tabular}} &
  LP &
  98.09$\pm$0.05 &
  88.43$\pm$0.25 &
  95.89$\pm$0.11 &
  91.67$\pm$0.50 &
  93.24$\pm$0.09 &
  93.04$\pm$0.34 &
  62.28$\pm$1.23 &
  81.70$\pm$0.23 &
  77.02$\pm$0.58 &
  93.44$\pm$0.09 &
  97.28$\pm$0.02 &
  77.02$\pm$1.25 &
  95.86$\pm$0.31 &
  71.00$\pm$0.50 &
  86.85 \\ 
 &
  MLP &
  97.52$\pm$0.14 &
  88.33$\pm$0.34 &
  95.54$\pm$0.40 &
  92.12$\pm$0.36 &
  93.41$\pm$0.09 &
  93.34$\pm$0.31 &
  63.11$\pm$0.84 &
  81.97$\pm$0.15 &
  77.81$\pm$0.64 &
  92.35$\pm$0.15 &
  97.38$\pm$0.01 &
  79.11$\pm$0.35 &
  96.54$\pm$0.05 &
  72.74$\pm$0.51 &
  87.23 \\
  & 
  Ours &
  \textbf{98.65$\pm$0.05} &
  \textbf{88.96$\pm$0.22} &
  \textbf{98.67$\pm$0.15} &
  \textbf{92.78$\pm$0.27} &
  \textbf{94.51$\pm$0.10} &
  \textbf{94.65$\pm$0.52} &
  \textbf{67.29$\pm$0.47} &
  \textbf{82.98$\pm$0.14} &
  \textbf{79.25$\pm$0.72} &
  \textbf{93.65$\pm$0.08} &
  \textbf{98.59$\pm$0.03} &
  \textbf{79.35$\pm$0.30} &
  \textbf{97.19$\pm$0.19} &
  \textbf{73.51$\pm$0.43} &
  \textbf{88.57} \\
\bottomrule
\end{tabular}%
}
\end{table}

\begin{table}[h]
\centering
\caption{Evaluation of our method on vision models in practice that are pre-trained on noisy datasets. We compare different methods on 4 DomainNet datasets for out-of-domain (OOD) evaluation. We perform training on either DomainNetSketch or DomainNetReal, and evaluate on DomainNetSketch, DomainNetReal, DomainNetPaining, DomainNetClipart without the training set. }
\label{tab:res-cv-ood}
\resizebox{0.5 \textwidth}{!}{%
\begin{tabular}{@{}l|l|ccc@{}}
\toprule
\multicolumn{1}{c|}{\begin{tabular}[c]{@{}c@{}}Pre-trained \\ Model\end{tabular}} &
  \multicolumn{1}{c|}{\begin{tabular}[c]{@{}c@{}}Tuning\\ Method\end{tabular}} &
  DomainNet Sketch &
  DomainNet Real &
  Avg \\ \midrule
\multirow{3}{*}{\begin{tabular}[c]{@{}l@{}}JFT-300M \\ Semi-Supervised\\ EfficientNet-B3\end{tabular}} &
  LP &
  46.22$\pm$6.17 &
  42.03$\pm$7.07 &
  44.13 \\
 &
  MLP &
  48.29$\pm$5.78 &
  43.61$\pm$7.53 &
  45.95 \\
 &
  Ours &
  \textbf{48.84$\pm$5.63} &
  \textbf{44.83$\pm$7.45} &
  \textbf{46.84} \\ \midrule
\multirow{3}{*}{\begin{tabular}[c]{@{}l@{}}ImageNet-21K\\ Fully Supervised\\ ResNetv2-152x2\end{tabular}} &
  LP &
  41.09$\pm$4.81 &
  40.55$\pm$7.89 &
  40.82 \\
 &
  MLP &
  41.98$\pm$5.08 &
  41.47$\pm$7.45 &
  41.73 \\
 &
  Ours &
  \textbf{42.68$\pm$4.85} &
  \textbf{42.15$\pm$7.23} &
  \textbf{42.42} \\ \midrule
\multirow{3}{*}{\begin{tabular}[c]{@{}l@{}}ImageNet-21K\\ Fully Supervised\\ Swin-L\end{tabular}} &
  LP &
  54.57$\pm$7.70 &
  47.19$\pm$7.45 &
  50.88 \\
 &
  MLP &
  53.81$\pm$6.01 &
  48.60$\pm$8.12 &
  51.21 \\
 &
  Ours &
  \textbf{55.68$\pm$5.48} &
  \textbf{49.01$\pm$6.15} &
  \textbf{52.35} \\ \midrule
\multirow{3}{*}{\begin{tabular}[c]{@{}l@{}}Laion-2B\\ CLIP\\ ConvNext-L\end{tabular}} &
  LP &
  66.66$\pm$7.69 &
  67.05$\pm$4.58 &
  66.86 \\
 &
  MLP &
  66.78$\pm$7.00 &
  70.07$\pm$4.90 &
  68.43 \\
 &
  Ours &
  \textbf{69.74$\pm$6.82} &
  \textbf{70.85$\pm$4.77} &
  \textbf{70.30} \\ \midrule
\multirow{3}{*}{\begin{tabular}[c]{@{}l@{}}Laion-2B\\ CLIP\\ ViT-L\end{tabular}} &
  LP &
  67.00$\pm$6.94 &
  66.77$\pm$4.74 &
  66.89 \\
 &
  MLP &
  68.99$\pm$6.59 &
  70.00$\pm$4.65 &
  69.50 \\
 &
  Ours &
  \textbf{70.48$\pm$6.91} &
  \textbf{70.45$\pm$4.98} &
  \textbf{70.47}
  \\ \bottomrule
\end{tabular}%
}
\end{table}

\subsection{Detailed Setup for Language Models Experiments}
\label{sec:append-exp-nlp-setup}

The model details for natural language processing are shown in \cref{tab:nlp-model-details}. 
We did not leverage larger language models mainly due to the limited computational resources. 
The recent open-sourced language models, such as Llama, have been trained on a very large-scale corpus of the web, 
evaluating them on GLUE and GLUE-X has the possibility to impose the problem of performing testing on the training samples.

\begin{table}[h]
\centering
\caption{Noisy language models we evaluated.}
\label{tab:nlp-model-details}
\resizebox{\textwidth}{!}{%
\begin{tabular}{@{}ccc@{}}
\toprule
Model & Pre-trained Data & Pre-trained Method \\ \midrule
BERT-L \citep{devlin2018bert}      &    BooksCorpus and d English Wikipedia            &      Masked Modeling \citep{devlin2018bert}                      \\
RoBERTa-L \citep{liu2019roberta}     &     BooksCorpus and d English Wikipedia        &               Masked Modeling  \citep{liu2019roberta}           \\ 
GPT-2  \citep{radford2019language} &       WebText        &      Autoregression        \\ 
text-ada-002     &          -  &            -         \\ 
\bottomrule
\end{tabular}%
}
\end{table}

Now, we present the dataset details here used in our analysis. 
For ID evaluation, we use CoLA, SST-2, MRPC, STS-B, QQP, MNLI, QNLI, and RTE tasks of GLUE benchmark \citep{2018glue}, as shown in \cref{tab:append-exp-nlp-id}. 
For OOD evaluation, following GLUE-X, we use Grammar Test \citep{yang2022glue} for CoLA, IMDB \citep{maas2011learning} for SST-2, QQP for MRPC, MNLI mismatched \citep{williams2017broad}, SNLI \citep{bowman2015large}, SICK \citep{zhang2018multi} for MNLI, Reconstructed NewsQA \citep{trischler2016newsqa} for QNLI, SciTail \citep{khot2018scitail} and HANS \citep{mccoy-etal-2019-right} for RTE, as shown in \cref{tab:append-exp-nlp-odd}.

\begin{table}[h]
\centering
\caption{Details of the 8 in-domain (ID) tasks of GLUE used to evaluate ID transfer performance.}
\label{tab:append-exp-nlp-id}
\resizebox{0.5 \textwidth}{!}{%
\begin{tabular}{l|cccc}
\toprule
\multicolumn{1}{c|}{Dataset} &  Classes & Train Size & Test Size & Evaluation Metric \\ \hline
CoLA                 &            2 & 8,500 & 1,000   &  matthews correlation           \\ 
SST-2                 &            2 & 67,000 & 1,800   &  accuracy          \\ 
MRPC                 &            2 & 3,700 & 1,700   &  accuracy          \\ 
STS-B                 &            5 & 7,000 & 1,400   &  pearson correlation          \\ 
QQP                &            2 & 364,000 & 391,000   &  accuracy          \\ 
MNLI                &            3 & 393,000 & 20,000   &  accuracy          \\ 
QNLI                &            2 & 105,000 & 5,400   &  accuracy          \\ 
RTE                &            2 & 2,500 & 3,000   &  accuracy          \\ 
\bottomrule
\end{tabular}%
}
\end{table}

\begin{table}[h]
\centering
\caption{Details of the out-of-domain (OOD) tasks of GLUE-X used to evaluate OOD transfer performance.}
\label{tab:append-exp-nlp-odd}
\resizebox{0.5 \textwidth}{!}{%
\begin{tabular}{l|ccc}
\toprule
\multicolumn{1}{c|}{Dataset} &  Classes  & Test Size & Evaluation Metric \\ \hline
Grammar Test                 &            2 &  304,277  &  matthews correlation           \\ 
IMDB                 &            2 &  50,000   &  accuracy          \\ 
MNLI mismatched                 &            2 &9,832   &  accuracy          \\ 
SNLI                 &            2 & 570,152    &  accuracy          \\
SICK                 &            2 &  9,840 &  accuracy          \\ 
NewsQA                &            2 &  119,525   &  accuracy          \\ 
SciTail                &            2 & 26,527   &  accuracy          \\ 
HANs                &            2 & 60,000   &  accuracy          \\ 
\bottomrule
\end{tabular}%
}
\end{table}

We use the AdamW optimizer and set the learning rate for LP as $0.01$ and for others as $0.001$ for all the experiments of language models. 
For LP, we do not use weight decay, and for others we use a weight decay of $0.0001$.
All tuning methods are trained for $10$ epochs with a linear learning rate scheduler.

\subsection{Detailed Results for Language Models Experiments}
\label{sec:append-exp-nlp-results}

The detailed ID and OOD results of language models evaluation are shown in \cref{tab:res-nlp-id} and \cref{tab:res-nlp-ood} respectively. 
NMTune outperforms LP and MLP tuning across all the tasks, whereas MLP tuning sometimes fall short than LP, demonstrating the necessitate of using the proposed regularization terms to help mitigate the effect of noise in pre-training and improve generalization performance. 

% {\floatsetup[table]{capposition=top}
\begin{table}[t!]
\centering
\caption{Evaluation of our method on language models in practice that are pre-trained on noisy datasets. We compare different methods on GLUE dev set for in-domain (ID) evaluation.}
\label{tab:res-nlp-id}
\resizebox{0.9 \textwidth}{!}{%
\begin{tabular}{@{}l|l|ccccccccl@{}}
\toprule
\multicolumn{1}{c|}{\multirow{2}{*}{Model}} &
  \multicolumn{1}{c|}{\multirow{2}{*}{Tuning}} &
  CoLA &
  MNLI &
  MRPC &
  QNLI &
  QQP &
  RTE &
  SST2 &
  STS &
  \multicolumn{1}{c}{\multirow{2}{*}{Avg}} \\
\multicolumn{1}{c|}{} &
  \multicolumn{1}{c|}{} &
  MCC &
  Acc &
  Acc &
  Acc &
  Acc &
  Acc &
  Acc &
  PCC &
  \multicolumn{1}{c}{} \\ \midrule
\multirow{3}{*}{BERT-L} &
  LP &
  46.18 &
  62.75 &
  72.05 &
  74.10 &
  84.83 &
  50.90 &
  88.19 &
  76.55 &
  69.44 \\
 &
  MLP &
  \textbf{46.99} &
  63.97 &
  72.30 &
  73.80 &
  84.88 &
  51.62 &
  88.30 &
  76.36 &
  69.78 \\
 &
  Ours &
  46.12 &
  \textbf{64.37} &
  \textbf{73.04} &
  \textbf{74.25} &
  \textbf{85.11} &
  \textbf{52.54} &
  \textbf{88.84} &
  \textbf{76.64} &
  \textbf{70.26} \\ \midrule
\multirow{3}{*}{RoBERTa-L} &
  LP &
  41.09 &
  59.27 &
  76.47 &
  76.07 &
  83.19 &
  55.96 &
  90.02 &
  75.93 &
  69.76 \\
 &
  MLP &
  42.93 &
  60.38 &
  76.22 &
  76.11 &
  82.94 &
  57.40 &
  90.25 &
  75.92 &
  70.27 \\
 &
  Ours &
  \textbf{43.91} &
  \textbf{60.59} &
  \textbf{77.69} &
  \textbf{76.33} &
  \textbf{83.30} &
  \textbf{58.96} &
  \textbf{90.71} &
  \textbf{76.24} &
  \textbf{70.97} \\ \midrule
\multirow{3}{*}{GPT-2} &
  LP &
  4.86 &
  53.11 &
  72.55 &
  67.65 &
  78.82 &
  56.68 &
  84.75 &
  40.93 &
  57.42 \\
 &
  MLP &
  4.46 &
  53.38 &
  73.53 &
  67.17 &
  78.72 &
  56.68 &
  84.75 &
  40.93 &
  57.19 \\
 &
  Ours &
  \textbf{6.41} &
  \textbf{54.21} &
  \textbf{73.77} &
  \textbf{68.09} &
  \textbf{78.95} &
  \textbf{57.07} &
  \textbf{85.14} &
  \textbf{41.09} &
  \textbf{58.09} \\ 
\midrule
\multirow{3}{*}{text-ada-002} &
  LP &
  22.92 &
  69.85 &
  64.74 &
  62.14 &
  74.96 &
  51.98 &
  91.05 &
  18.04 &
  56.96 \\
 &
  MLP &
  33.90 &
  70.49 &
  66.42 &
  69.54 &
  84.28 &
  52.34 &
  91.85 &
  42.28 &
  63.89 \\
 &
  Ours &
  \textbf{36.96} &
  \textbf{72.05} &
  \textbf{70.34} &
  \textbf{70.25} &
  \textbf{85.54} &
  \textbf{54.51} &
  \textbf{92.89} &
  \textbf{45.39} &
  \textbf{65.99} \\ 

\bottomrule
\end{tabular}%
}
\end{table}

% {\floatsetup[table]{capposition=top}
\begin{table}[t!]
\centering
\caption{Evaluation of our method on language models in practice that are pre-trained on noisy datasets. We compare different methods on GLUE-X for ouf-of-domain (OOD) evaluation.}
\label{tab:res-nlp-ood}
\resizebox{0.9 \textwidth}{!}{%
\begin{tabular}{@{}l|l|ccccccccl@{}}
\toprule
\multicolumn{1}{c|}{\multirow{2}{*}{Model}} &
  \multicolumn{1}{c|}{\multirow{2}{*}{Tuning}} &
  CoLA &
  MNLI &
  MRPC &
  QNLI &
  QQP &
  RTE &
  SST2 &
  STS &
  \multicolumn{1}{c}{\multirow{2}{*}{Avg}} \\
\multicolumn{1}{c|}{} &
  \multicolumn{1}{c|}{} &
  MCC &
  Acc &
  Acc &
  Acc &
  Acc &
  Acc &
  Acc &
  PCC &
  \multicolumn{1}{c}{} \\ \midrule
\multirow{3}{*}{BERT-L} &
  LP &
  13.71 &
  36.82 &
  55.85 &
  63.60 &
  53.14 &
  50.67 &
  73.66 &
  57.81 &
  50.65 \\
 &
  MLP &
  14.11 &
  36.49 &
  56.15 &
  63.61 &
  52.34 &
  50.02 &
  73.32 &
  58.91 &
  50.62 \\
 &
  Ours &
  \textbf{14.57} &
  \textbf{37.62} &
  \textbf{56.68} &
  \textbf{63.88} &
  \textbf{55.17} &
  \textbf{50.98} &
  \textbf{74.52} &
  \textbf{59.61} &
  \textbf{51.63} \\ \midrule
\multirow{3}{*}{RoBERTa-L} &
  LP &
   24.07  &
   37.05 &
   48.51 &
   57.83 &
   24.93 &
   51.02 &
   71.24 &
   41.74 &
   44.55 \\
 &
  MLP &
  24.50 &
  37.32 &
  48.96 &
  58.56 &
  24.12 &
  52.51 &
  73.86 &
  41.95 &
  45.22 \\
  &
  Ours &
  \textbf{25.29} &
  \textbf{37.84} &
  \textbf{49.52} &
  \textbf{59.72} &
  \textbf{26.78} &
  \textbf{53.19} &
  \textbf{81.42} &
  \textbf{42.29} &
  \textbf{47.01} \\ \midrule
\multirow{3}{*}{GPT-2} &
  LP &
  4.12 &
  24.93 &
  45.24 &
  54.00 &
  16.22 &
  49.50 &
  53.75 &
  45.68 &
  36.68 \\
 &
  MLP &
  4.89 &
  25.20 &
  47.99 &
  54.11 &
  17.21 &
  49.71 &
  53.60 &
  45.21 &
  37.24 \\
 &
  Ours &
  \textbf{5.31} &
  \textbf{32.56} &
  \textbf{49.78} &
  \textbf{55.97} &
  \textbf{17.34} &
  \textbf{49.96} &
  \textbf{54.28} &
  \textbf{47.39} &
  \textbf{39.07} \\ 
\midrule
\multirow{3}{*}{text-ada-002} &
  LP &
   8.06 &
   65.14&
   38.66 &
   58.12 &
   32.60 &
   51.53 &
   84.07 &
   14.30 &
   44.06 \\
 &
  MLP &
   15.47 &
   67.23 &
   44.91 &
   63.59 &
   50.24 &
   51.44 &
   83.11 &
   34.46 &
   51.31 \\
 &
  Ours &
  \textbf{17.50} &
  \textbf{68.97} &
  \textbf{46.41} &
  \textbf{63.81} &
  \textbf{55.34} &
  \textbf{52.81} &
  \textbf{85.16} &
  \textbf{37.80} &
  \textbf{53.48} \\ 

\bottomrule
\end{tabular}%
}
\end{table}

\subsection{Transferring on Noisy Downstream Datasets}
\label{sec:append-exp-noise}

We additionally study the setting where both pre-training and downstream datasets contain noisy labels. 
For pre-training noise, we use the ResNet-50 models pre-trained on noisy ImageNet-1K and YFCC15M with different noise ratios $\gamma \in \{0\%, 5\%, 10\%, 20\%, 30\%\}$, as in \cref{sec:understand}. 
For downstream noise, we adopt synthetic noise CIFAR-10 and CIFAR-100 which are usually used in noisy label learning \citep{sopliu22w,chen2023imprecise}. 
We generate symmetric label noise by uniformly flipping labels for a percentage of the training set for all classes.
We denote the noise ratio of downstream datasets as $\eta$, and set it to $\{0\%, 10\%, 20\%, 30\%, 40\%, 50\%\}$. 
We compare LP and NMTune in this setting, as shown in \cref{fig:append-noise-lp} and \cref{fig:append-noise-nml}, respectively. 

On the LP results in \cref{fig:append-noise-lp}, we find similar observations as our analysis in \cref{sec:understand}, where the $5\%$ and $10\%$ noisy pre-trained models usually outperforms the clean pre-trained model on downstream tasks, even the downstream tasks contain different level of noise. 
It indicates that the same conclusion from our main paper may extend and generalize to noisy downstream tasks, which highlights the importance of the proposed new topic - Noisy Model Learning - as the complementary to noisy label learning. 

\begin{figure}[!t]
\centering
    \hfill
    \subfigure[IN-1K CIFAR10]{\label{fig:append-noise-lp-in1k-c10}\includegraphics[width=0.24\linewidth]{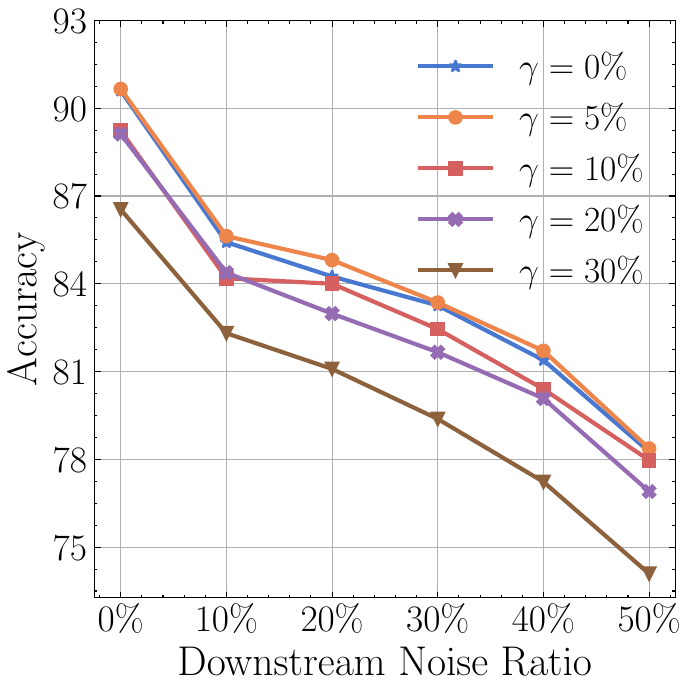}}
    \hfill
    \subfigure[IN-1K CIFAR100]{\label{fig:append-noise-lp-in1k-c100}\includegraphics[width=0.24\linewidth]{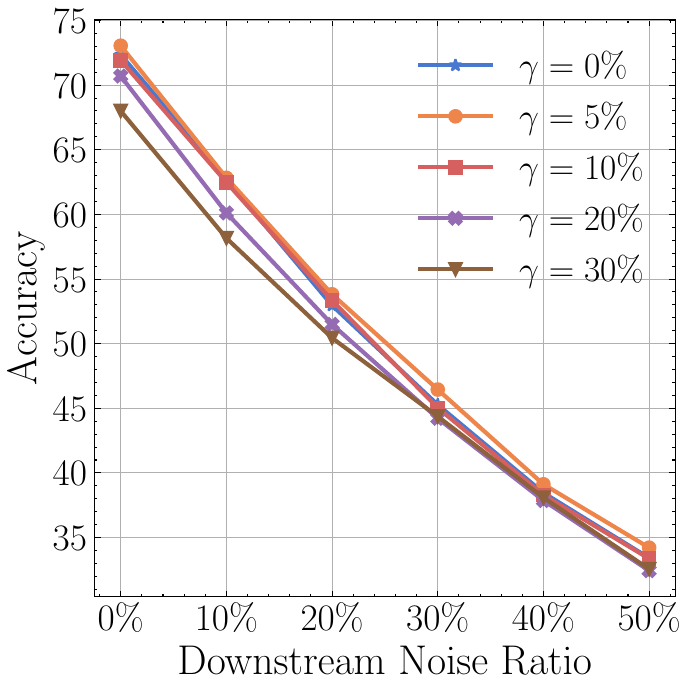}}
    \hfill
    \subfigure[YFCC15M CIFAR10]{\label{fig:append-noise-lp-yfcc-c10}\includegraphics[width=0.24\linewidth]{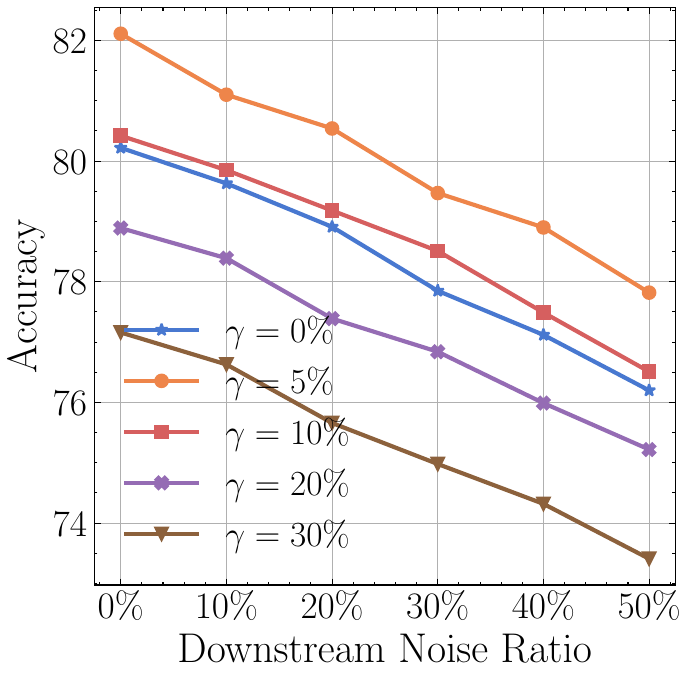}}
    \hfill
    \subfigure[YFCC15M CIFAR100]{\label{fig:append-noise-lp-yfcc-c100}\includegraphics[width=0.24\linewidth]{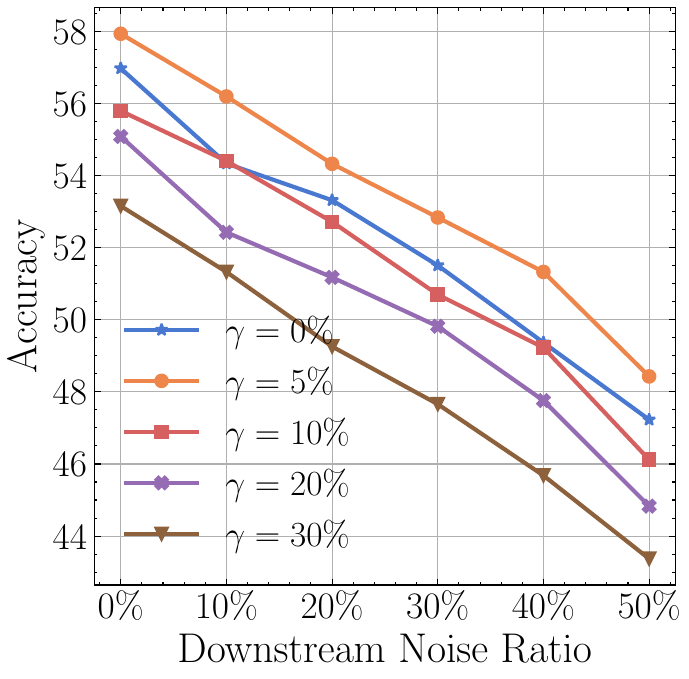}}
    \hfill
\caption{Linear Probing of noisy ResNet-50 models on noisy CIFAR-10 and CIFAR-100.} 
\label{fig:append-noise-lp}
\end{figure}

More importantly, we find that the proposed NMTune method has similar mitigation effect on noisy downstream tasks as the clean ones. 
On the NMTune results in \cref{fig:append-noise-nml}, we show that the clean pre-trained models now produce superior performance compared to noisy pre-trained models by utilizing the proposed regularization terms. 
It also improves the general performance when the noise ratio in downstream tasks is light, e.g., smaller than $40\%$. 
When the noise ratio in downstream tasks further increases, the performance of NMTune fall shorts to LP, which is acceptable because the regularization terms are not designed to be noise-tolerant. 
Noteworthy is that, even with slightly worse performance than LP, the performance of clean pre-trained mode still stays the best with NMTune. 
Devising NMTune to be more noise-tolerant on downstream tasks and experiments on practical asymmetric and instance-dependent noise \citep{wei2021learning} would be very interesting and leave for the future exploration.

\begin{figure}[!t]
\centering
    \hfill
    \subfigure[IN-1K CIFAR10]{\label{fig:append-noise-nml-in1k-c10}\includegraphics[width=0.24\linewidth]{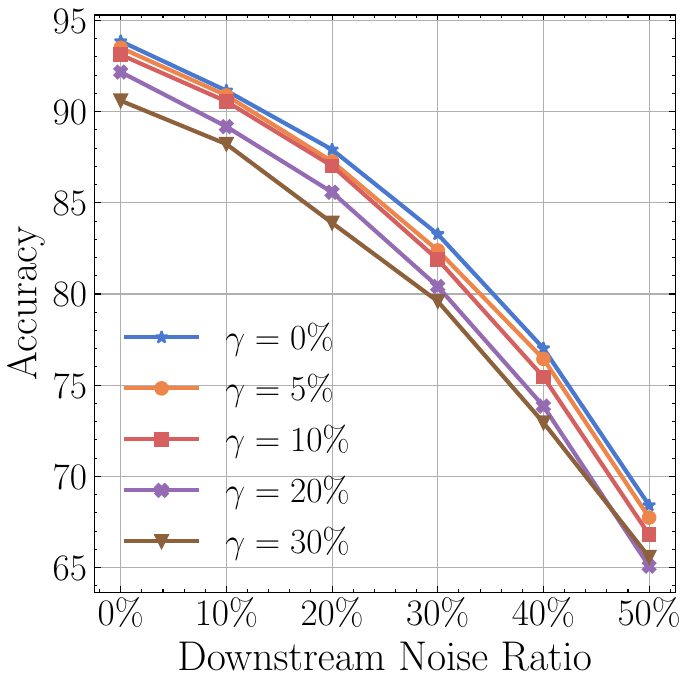}}
    \hfill
    \subfigure[IN-1K CIFAR100]{\label{fig:append-noise-nml-in1k-c100}\includegraphics[width=0.24\linewidth]{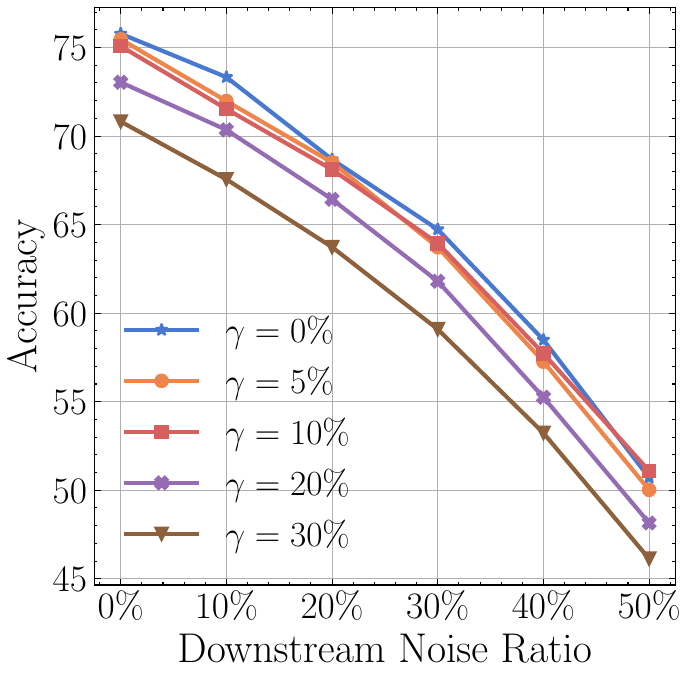}}
    \hfill
    \subfigure[YFCC15M CIFAR10]{\label{fig:append-noise-nml-yfcc-c10}\includegraphics[width=0.24\linewidth]{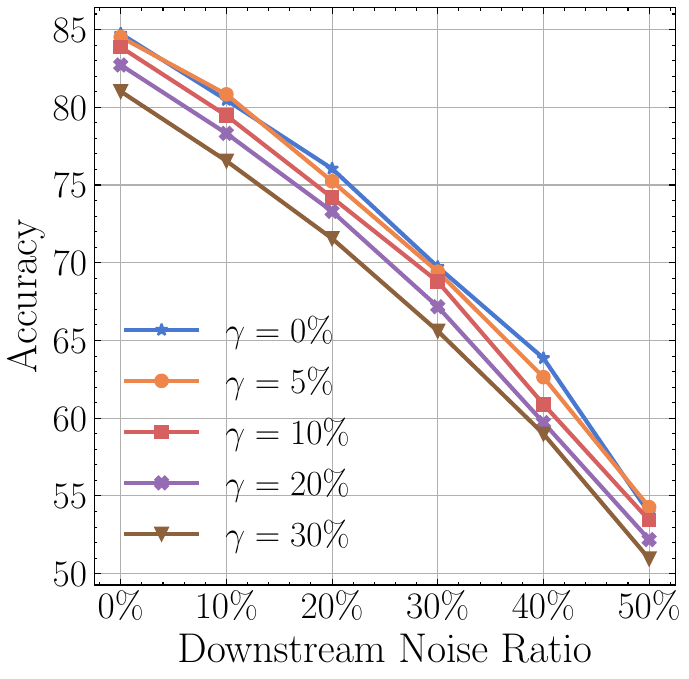}}
    \hfill
    \subfigure[YFCC15M CIFAR100]{\label{fig:append-noise-nml-yfcc-c100}\includegraphics[width=0.24\linewidth]{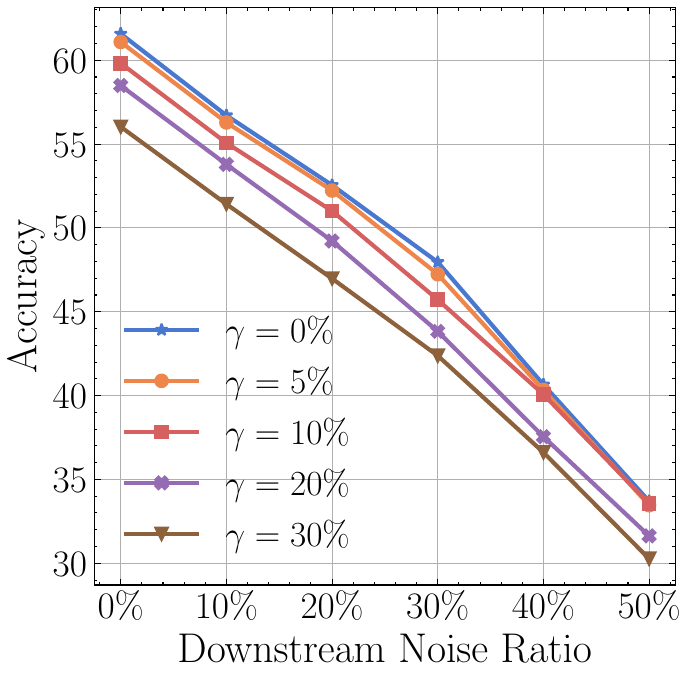}}
    \hfill
\caption{NMTune of noisy ResNet-50 models on noisy CIFAR-10 and CIFAR-100.} 
\label{fig:append-noise-nml}
\end{figure}

\subsection{Runtime Analysis}
\label{sec:append-exp-runtime}

The runtime analysis for NMTune, in comparison to LP and MLP tuning is shown in \cref{tab:append-exp-runtime}.  All of our experiments on downstream are conducted on single NVIDIA V100 GPU.
Thus we report the average GPU hours for running the ID and OOD evaluation of vision and language tasks. 
From the results, the proposed NMTune introduces minimal computation, compared to MLP with the exactly the same parameters. 
The additional computation burden may involve in the SVD calculation and the covariance matrix calculation on the features.

\input{tables/tb-runtime}

\subsection{Ablation Study}
\label{sec-append-exp-ablation}

The ablation study of NMTune is present here, where we run evaluation on the ID vision datasets. 
We use three ResNet-50 models from ImageNet-1K pre-training and YFCC15M pre-training for ablation, including the clean pre-trained, $5\%$ noise pretrained, and $10\%$ noise pretrained.

We study the MLP architecture, more specifically, the non-linearity and the number of layers in MLP in \cref{tab:ablation-mlp}.
From the results, one can observe that removing the non-linearity reduces the performance significantly. 
Adding more layers only improves the performance slightly but introduces much more parameters. 
Thus we adopt the 2-layer MLP architecture with ReLU activation. 
The overall structure is shown in \cref{fig:mlp-arch}.

\begin{table}[h]
\centering
\caption{Ablation study of MLP architecture on ID vision datasets.}
\label{tab:ablation-mlp}
\resizebox{0.6 \textwidth}{!}{%
\begin{tabular}{@{}cc|c|c|c@{}}
\toprule
\multirow{2}{*}{MLP Layers} & \multirow{2}{*}{Activation} & \multirow{2}{*}{Models} & IN-1K Pre-trained & YFCC15M Pre-trained \\
                   &                       &    & ID Accuracy & ID Accuracy \\ \midrule
\multirow{3}{*}{2} & \multirow{3}{*}{ReLU} & 0  &   75.06          &     67.34        \\
                   &                       & 5  &   74.87          &      67.44       \\
                   &                       & 10 &   74.27          &     66.95        \\ \midrule
\multirow{3}{*}{2} & \multirow{3}{*}{None} & 0  &   73.83          &      65.62       \\
                   &                       & 5  &   74.17         &        66.14     \\
                   &                       & 10 &   73.39          &       65.51      \\ \midrule
\multirow{3}{*}{3} & \multirow{3}{*}{ReLU} & 0  &    75.16         &     67.56        \\
                   &                       & 5  &     74.99        &     67.49        \\
                   &                       & 10 &     74.48        &     67.13        \\ \midrule
\multirow{3}{*}{4} & \multirow{3}{*}{ReLU} & 0  &     75.13        &     67.51        \\
                   &                       & 5  &     74.92        &      67.48       \\
                   &                       & 10 &     74.14  &            67.02 \\ \bottomrule
\end{tabular}%
}
\end{table}

\begin{figure}
    \centering
    \includegraphics[width=0.2\textwidth]{figures/mlp_arch.pdf}
    \caption{Architecture of the 2-layer MLP with ReLU activation.}
    \label{fig:mlp-arch}
\end{figure}

We also conduct ablation on the loss weight of different regularization terms we proposed in \cref{tab:ablation-loss}. 
From the results, we find that the proposed covariance regularization $\mathcal{L}_{\mathrm{COV}}$ in general rectifies the effect of noise, improving the performance of clean pre-trained models to achieve better results than noisy pre-trained models. 
We can also observe that the dominant singular value regularization $\mathcal{L}_{\mathrm{SVD}}$ helps improve generalization. 
Solely adding $\mathcal{L}_{\mathrm{MSE}}$ or $\mathcal{L}_{\mathrm{SVD}}$ does not produces this behavior and yields slight worse results.

\begin{table}[h]
\centering
\caption{Ablation study of different loss weights on ID vision datasets}
\label{tab:ablation-loss}
\resizebox{0.6 \textwidth}{!}{%
\begin{tabular}{@{}ccc|c|c|c@{}}
\toprule
\multirow{2}{*}{$\mathcal{L}_{\mathrm{MSE}}$}  & \multirow{2}{*}{$\mathcal{L}_{\mathrm{COV}}$}  & \multirow{2}{*}{$\mathcal{L}_{\mathrm{SVD}}$}  & \multirow{2}{*}{Models} & \multicolumn{1}{c|}{IN-1K Pre-trained} & YFCC15M Pre-trained \\
                      &                       &                       &    & \multicolumn{1}{c|}{ID Accuracy} & ID Accuracy \\ \midrule
\multirow{3}{*}{0.01} & \multirow{3}{*}{0.01} & \multirow{3}{*}{0.01} & 0                       &  75.06                  &     67.34                \\
                      &                       &                       & 5  &    74.87      &      67.44         \\
                      &                       &                       & 10 &  74.27        &      66.95       \\ \midrule
\multirow{3}{*}{0.00} & \multirow{3}{*}{0.01} & \multirow{3}{*}{0.01} & 0  &         74.34                       &       66.59   \\
                      &                       &                       & 5  &          74.18                         &       66.54      \\
                      &                       &                       & 10 &            74.09                    &     66.17        \\ \midrule
\multirow{3}{*}{0.01} & \multirow{3}{*}{0.00} & \multirow{3}{*}{0.01} & 0  &        73.65                          &      65.41     \\
                      &                       &                       & 5  &         74.23                           &     66.02       \\
                      &                       &                       & 10 &        73.56                          &     65.39        \\ \midrule
\multirow{3}{*}{0.01} & \multirow{3}{*}{0.00} & \multirow{3}{*}{0.00} & 0  &       74.16                             &       66.27      \\
                      &                       &                       & 5  &        74.24                           &       66.31      \\
                      &                       &                       & 10 &        73.17                           &        66.08     \\ \midrule
  \multirow{3}{*}{0.01} & \multirow{3}{*}{0.01} & \multirow{3}{*}{0.00} & 0  &      74.74                            &        67.03     \\
                      &                       &                       & 5  &        74.32                       & 66.83            \\
                      &                       &                       & 10 &        73.92                         
 &        66.70     \\ \midrule
\multirow{3}{*}{0.00} & \multirow{3}{*}{0.01} & \multirow{3}{*}{0.00} & 0  &       74.41                           &     66.51        \\
                      &                       &                       & 5  &        74.20                          &        66.47     \\
                      &                       &                       & 10 &           73.98                       &        66.12     \\ \midrule
\multirow{3}{*}{0.00} & \multirow{3}{*}{0.00} & \multirow{3}{*}{0.01} & 0  &           72.21                       &      65.08       \\
                      &                       &                       & 5  &              73.49                    &     65.24        \\
                      &                       &                       & 10 &           72.87                       &       64.76      \\ \hline
\multirow{3}{*}{0.00} & \multirow{3}{*}{0.00} & \multirow{3}{*}{0.00} & 0  &       73.96                           &       66.11      \\
                      &                       &                       & 5  &          73.97                        &     66.19        \\
                      &                       &                       & 10 &       73.13                           &     65.93        \\                       
\bottomrule
\end{tabular}%
}
\end{table}

\revision{

\section{More Discussions}

More discussions about our work are provided here.

\subsection{Limitations}

The limitation mainly lies in our empirical study of the noise in pre-training. 
Due to the limited computing resources, we could only conduct experiments on reltively small scale backbone and datasets, while most of the SOTA foundation models are of much more parameters and are trained on much larger datasets. 
Also, the empirical experiments is limited to actual supervised pre-training. 
Other pre-training objectives will be explored in our future work. 
That being said, we do believe the observation and conclusions from our practical experiments could scale and extend to larger datasets, stronger backbones, and other training objectives.

\subsection{Potential Failure}

We do observe some failure cases of the proposed methods. 
For example, from the results in Table.7, the proposed method falles short to LP on Caltech101 on almost all backbones we studied, while improving over MLP. 
Our hypothesis for the failure is that the SVD regularization term in the proposed method might need to optimize the top-K singular values instead of just the largest one. The optimal value of K might be different dataset. However, setting $K=1$ can already achieves reasonable performance for most of the tasks.

}
